# Supplementary material for: DeGPR: Deep Guided Posterior Regularization for Multi-Class Cell Detection and Counting
Source: arXiv:2304.00741 source file (2023-04-03)
Supplement: Supplementary file 1 [file Supplimentary.tex]

% CVPR 2023 Paper Template
% based on the CVPR template provided by Ming-Ming Cheng (https://github.com/MCG-NKU/CVPR_Template)
% modified and extended by Stefan Roth (stefan.roth@NOSPAMtu-darmstadt.de)

\documentclass[10pt,twocolumn,letterpaper]{article}

%%%%%%%%% PAPER TYPE  - PLEASE UPDATE FOR FINAL VERSION
% \usepackage[review]{cvpr}      % To produce the REVIEW version
% \usepackage{cvpr}              % To produce the CAMERA-READY version
\usepackage[pagenumbers]{cvpr} % To force page numbers, e.g. for an arXiv version

% Include other packages here, before hyperref.
\usepackage{graphicx}
\usepackage{amsmath}
\usepackage{amssymb}
\usepackage{booktabs}
\usepackage{tikz}
\usepackage{float}
\usepackage{algorithm}
\usepackage{algorithmic}
\usepackage[accsupp]{axessibility}
% It is strongly recommended to use hyperref, especially for the review version.
% hyperref with option pagebackref eases the reviewers' job.
% Please disable hyperref *only* if you encounter grave issues, e.g. with the
% file validation for the camera-ready version.
%
% If you comment hyperref and then uncomment it, you should delete
% ReviewTempalte.aux before re-running LaTeX.
% (Or just hit 'q' on the first LaTeX run, let it finish, and you
%  should be clear).
\usepackage[pagebackref,breaklinks,colorlinks]{hyperref}

% Support for easy cross-referencing
\usepackage[capitalize]{cleveref}
\crefname{section}{Sec.}{Secs.}
\Crefname{section}{Section}{Sections}
\Crefname{table}{Table}{Tables}
\crefname{table}{Tab.}{Tabs.}

%%%%%%%%% PAPER ID  - PLEASE UPDATE
 % *** Enter the CVPR Paper ID here

\begin{document}

\newcommand{\sys}{\textsc{DeGPR}}

%%%%%%%%% TITLE - PLEASE UPDATE
\title{\sys: Deep Guided Posterior Regularization\\ for Multi-Class Cell Detection and Counting}

\author{
Aayush Kumar Tyagi$^{1*}$, Chirag Mohapatra$^{1*}$, Prasenjit Das$^{3}$,
Govind Makharia$^{3}$,\\  
Lalita Mehta$^{3}$, Prathosh AP$^{2}$, Mausam$^{1}$\\
% $^{1}$Indian Institute of Technology, Delhi ~~~~~~$^{2}$Indian Institute of Science, Bangalore\\
% $^{3}$All India Institute of Medical Sciences, New Delhi
$^{1}$IIT Delhi ~~~~~~$^{2}$IISc, Bangalore
~~~~~~$^{3}$AIIMS, New Delhi\\
{\small \{tyagiaayushkumar, chirag131020, prasenaiims, govindmakharia,  mehralalita9910, prathoshap\}@gmail.com, mausam@cse.iitd.ac.in
}
}
\maketitle
\def\thefootnote{*}\footnotetext{Equal contribution}
\section{Dataset details}
Table \ref{tab: Annotations} provides the annotation number for each class of the MuCeD dataset.
\begin{table}[h]
    \caption{Annotation numbers}
    \centering
    \setlength{\tabcolsep}{3pt}
    \begin{tabular}{p{30pt} p{120pt} p{35pt} }
        \hline
        S.No & Tissue Name& Annotated \\
        \hline
        1 & Intra-Epithelial Lymphocyte &2090\\
        2&Epithelial Nuclei&6518\\
        \hline
    \end{tabular}
    \label{tab: Annotations}
\end{table}

Fig \ref{fig:dataset} provides the details of how whole slide image (WSI) is sliced to get the image sub-slices. Here, it is important to note that we mask out region apart from the annotated epithelial area. Epithelial area is shown in fig \ref{fig:dataset} as bold boundary of the villi. We select good villi based on continuity of epithelial layer for our analysis. Further, image is sliced into 9 sub-images, where each dimension is 640 $\times$ 640.

\begin{figure}[h!]
    \centering
    \includegraphics[scale = 0.23]{DeGPR/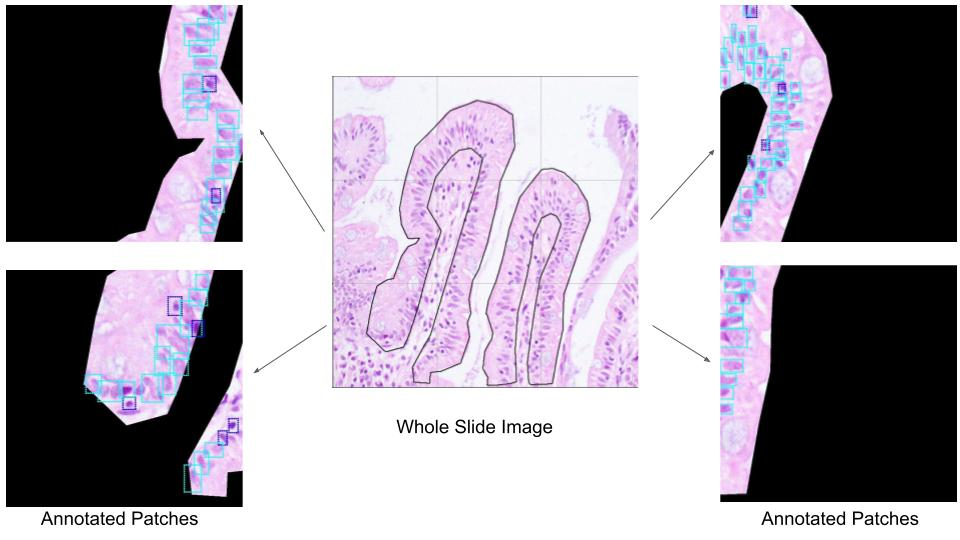}
    \caption{Fig shows sample image of celiac dataset. Each WSI image is sliced into 9 parts and further rescaled to improve the magnification of cells. IELs are marked in violet bounding boxes. and Epithelial nuclei are marked in cyan bounding boxes}
    \label{fig:dataset}
\end{figure}

\section{Training Object detection model}
We tested DeGPR on multiple object detection models to verify if it is object agnostic. Yolov5 is from the class of single stage object detectors. Yolo slices the images into multiple grids and corresponding to each grid, it predicts the bounding boxes with confidence score and class probability map. Faster-RCNN introduced a region proposal network (RPN) to make computation of region proposals cost effective. RPN can be trained end-to-end to generate high quality proposals. EfficientDet introduced Bi-directional feature pyramid network (BiFPN) and compound scaling to uniformly scale depth, width and resolution. \\
For experimentation, we use official implementation of Yolov5 \footnote{https://github.com/ultralytics/yolov5} and Faster-RCNN using are in pytorch. We use pytorch implementation of EfficientDet \footnote{https://github.com/rwightman/efficientdet-pytorch} with pre-trained model efficientdet d0. \\ 
We believe that EfficientDet has more parameters and easily overfits on small datasets, hence the performance of EfficientDet is comparitively lower than Yolo and FasterRCNN. 
We pre-trained model with Kaggle cell segmentation dataset. However, with CoNSeP and MoNuSac, we did not see improvements with pre-training, since they both have much more training data than MuCeD.
DeGPR creates a computation overhead for training GMM $G(\theta)$ for mini-batch. This results in increased training time upto 1.5 hour in addition to baseline training time. Yolov5 takes 3-4 hour to complete the training process depending on early stop. Faster-RCNN takes 6-7 hours with DeGPR and EfficientDet takes 8-10 hours to complete the training process. All experiments were preformed on NVIDIA-RTX 5000.
We found p values of 0.008 and 0.007 for Precision and mAP with MuCeD using student’s paired t-test. While performing ablation study, we did experiments with only size (mAP
020 0.773) and only intensity (mAP 0.770), and observed that combined size and intensity performs better (mAP 0.779).

\section{Training Contrastive encoder}
Fig \ref{fig:Contrastive_plot} provide the t-SNE plot of the trained Encoder for one of the fold of the MuCeD dataset. As we know encoder $E(\theta)$ is trained with supervised constrastive loss ($L_{SupCon}$). Contrastive encoding enforces similar data points to be close. We can see from the fig \ref{fig:Contrastive_plot}, IEL's (red) and EN (blue) are represented by separate clusters. Hence, encoder $E(\theta)$ is able to learn the discriminative features between the cell types.

\begin{figure}[h!]
    \centering
    \includegraphics[scale = 0.5]{DeGPR/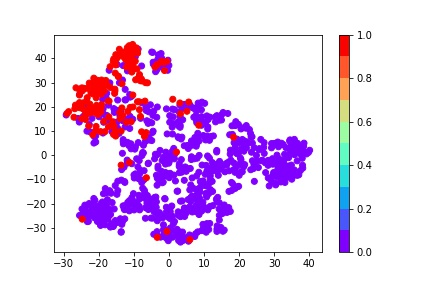}
    \caption{t-SNE plot of embeddings learnt for IEL's (red) and EN (blue). We can see from the embeddings that two clusters are formed which meant that model is able to map similar embeddings close to each other.}
    \label{fig:Contrastive_plot}
\end{figure}

Tab \ref{tab:Ablation} provide comparative analysis for different encoder backbones like ResNet 18, 34, 50, 101. We observed that larger models does not provide any additional performance gain hence we used ResNet18 for our experimentation purpose.
\begin{table}[t]
\caption{Ablation for Encoder$E_{\phi}$}
\centering
\setlength{\tabcolsep}{4pt}
\begin{tabular}{p{40pt} p{38pt} p{38pt} p{30pt} p{30pt}}
\hline
Model & Acc & Precision&Recall&F1 \\
\hline
ResNet18 & 0.867 & 0.938 & 0.740& 0.827\\
\hline
ResNet34& 0.8564 & 0.931&  0.6455 & 0.762\\
\hline
ResNet50& 0.8604 & 0.946 & 0.661 & 0.778\\
\hline
ResNet101& 0.859 & 0.929 & 0.73 & 0.817\\
\hline
\end{tabular}
\label{tab:Ablation}
\end{table}

\section{Counting via detection}
Table \ref{tab:Counting_vs_Localisation_MoNuSAC} compares counting via detection with density map based methods for MoNuSAC dataset. We observe from tab \ref{tab:Counting_vs_Localisation_MoNuSAC} Yolov5 with \sys{} is performing well for most of the cell types. 
\begin{table}[H]
\caption{Counting vs Localization (MoNuSAC)}
\setlength{\tabcolsep}{3pt}
\begin{tabular}{p{45pt} p{35pt} p{35pt} p{40pt} p{30pt} p{20pt} }
\hline
Model& MAE Epith& MAE Lympho & MAE Neutro & MAE Macro& MAE Avg\\
\hline
UNet&57.64&33.91&1.31&2.55&23.85\\
FCRN-A&64.48&60.71&\textbf{0.17}&1.52&31.72\\
SAU-Net&60.42&54.42&1.49&2.72&29.76\\
% yolov5&10.25&41.49&19.09&19.40\\
Yolov5 (DeGPR)& \textbf{12.01}& \textbf{10.69}& 0.81& \textbf{2.32}&\textbf{6.46} \\
\hline

\end{tabular}
\label{tab:Counting_vs_Localisation_MoNuSAC}
\end{table}

For the density map based methods, we trained separate models for each class type.
We can see that Yolov5 with DeGPR has the best performance.

\section{Visualization}
Fig \ref{fig: bbox_prediction_MuCeD_sup}, \ref{fig: bbox_prediction_CoNSeP} and \ref{fig: bbox_prediction_MoNuSAC} provide the qualitative analysis of the model performance on MuCeD, CoNSeP and MoNuSAC respectively. The first column shows the raw images, the second column shows the images with ground truth bounding boxes, the third column shows the performance of the baseline Yolov5 model while the final column shows the performance of the Yolov5 model with \sys{}. We can see that \sys{} helps in solving problems like extra detections, missed detections and misclassifications.

Fig \ref{fig:tSNE_imp_vs_exp} is a t-SNE plot for implicit vs explicit features. We can see from the fig \ref{fig:tSNE_imp_vs_exp} implicit and explict features do not overlap completely and are actually capture complementary information.
\begin{figure}
    \centering
    \includegraphics[scale = 0.3]{DeGPR/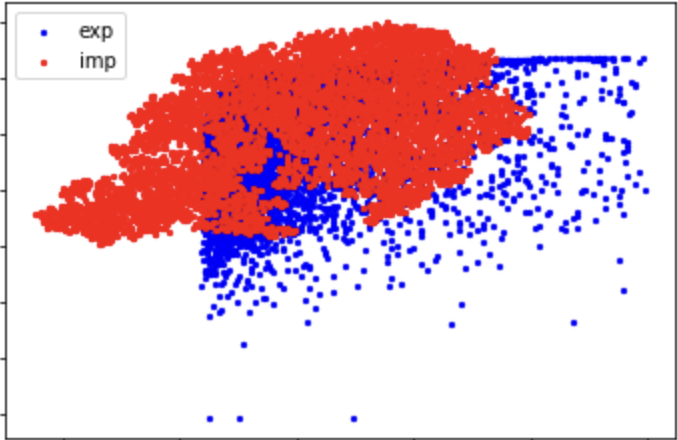}
    \caption{Implicit and explicit features}
    \label{fig:tSNE_imp_vs_exp}
\end{figure}

\section{Convergence of losses}
Fig \ref{fig:convergence_gmm} provide loss convergence for detection loss ($\mathcal{L}_{det}$), classification loss ($\mathcal{L}_{cls}$) and DeGPR ($\mathcal{L}_{reg}$). We can observe from the fig \ref{fig:convergence_gmm} that all loss converge over the epochs.
\begin{figure}[h!]
    \centering
    \includegraphics[scale = 0.2]{DeGPR/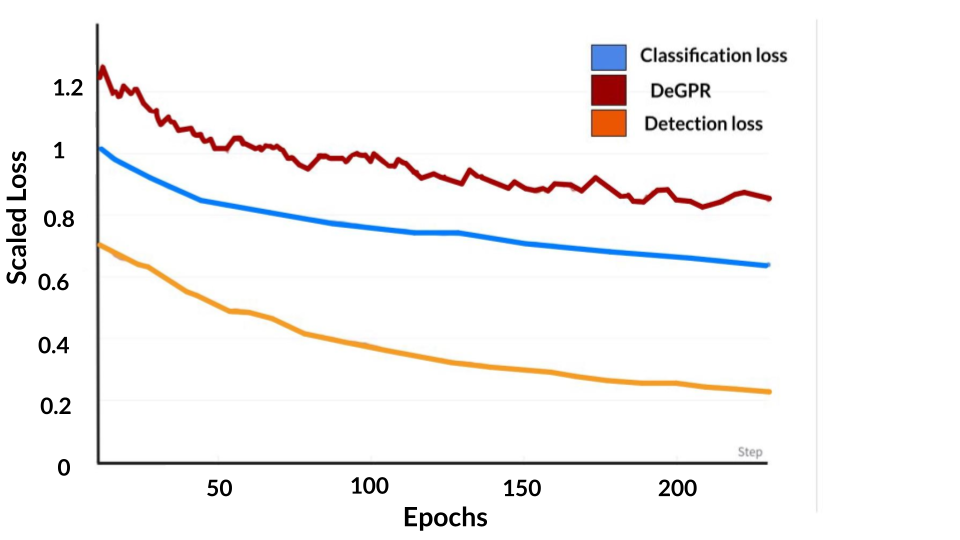}
    \caption{Convergence of losses. }
    \label{fig:convergence_gmm}
\end{figure}

\section{SOTA comparision}
We compared our method with MCSpatNet. MCSpatNet is a dot-annotation method, so we were only able to add DEGPR with intensity feature.  
On ConSeP, stomal cell predictions gained 7.7 F1 points, due to intensity differences captures by DEGPR Tab \ref{tab:SOTA Consep}. Because MCSpatNet uses spatial information to cluster cells, it fails to perform well on MuCeD (0.549 mean F1, compared 078 to 0.742 for Yolo+DEGPR), because here, IELs and ENs are interspersed across the region as shown in Tab \ref{tab:SOTA MuCeD}.
Another method HoverNet uses segmentation based annotation. We experimented with CoNSeP Tab \ref{tab:SOTA_hovernet}, and found that DEGPR yields negligible improvements (but doesn’t hurt performance), probably because vital information of shape is already captured by the base model.
\begin{table}[t]
\caption{F score of individual classes for MuCeD dataset}
\centering
\setlength{\tabcolsep}{4pt}
\begin{tabular}{p{90pt} p{38pt} p{38pt}}
\hline
Model & IEL & Epith\\
\hline
MCSpatNet & 0.545 & 0.554 \\
\hline
\sys & \textbf{0.725} & \textbf{0.759}\\
\hline
\end{tabular}
\label{tab:SOTA MuCeD}
\end{table}

\begin{table}[t]
\caption{F score of individual classes for CoNSeP dataset}
\centering
\setlength{\tabcolsep}{4pt}
\begin{tabular}{p{90pt} p{20pt} p{20pt} p{20pt}}
\hline
Model & Infl. & Epi.& Sto.\\
\hline
MCSpatNet & 0.724 & 0.695 & 0.682\\
\hline
\sys & 0.731 & 0.632& 0.538\\
\hline
MCSpatNet(\sys) & \textbf{0.736} & \textbf{0.698} & \textbf{0.759}\\
\hline
\end{tabular}
\label{tab:SOTA Consep}
\end{table}

\begin{table}[t]
\caption{Comparative analysis with HoverNet for CoNSeP}
\centering
\setlength{\tabcolsep}{4pt}
\begin{tabular}{p{40pt} p{30pt} p{30pt}p{30pt}p{30pt}p{30pt}}
\hline
Model & Dice & AJI& DQ & SQ& PQ\\
\hline
HoverNet & 0.853&0.531&0.702&0.778&0.547\\
\hline
Reprod. & 0.838&0.534&0.652&0.764&0.499\\
\hline
\sys& 0.838&0.533&0.655&0.764&0.502\\
\hline
\end{tabular}
\label{tab:SOTA_hovernet}
\end{table}

\begin{figure*}
\centering
\begin{tikzpicture}[scale=1.03,transform shape, picture format/.style={inner sep=1pt}]

  \node[picture format]                   (A1)   at (0,0)            {\includegraphics[width=1.6in, height = 1.6in]{DeGPR/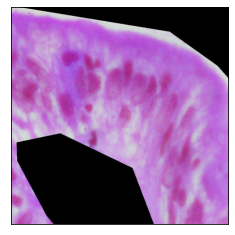}};
  \node[picture format,anchor=north]      (B1) at (A1.south) {\includegraphics[width=1.6in, height = 1.6in]{DeGPR/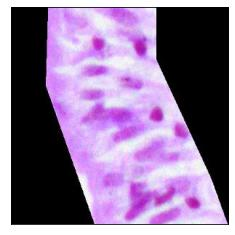}};
  \node[picture format,anchor=north]      (C1) at (B1.south) {\includegraphics[width=1.6in, height = 1.6in]{DeGPR/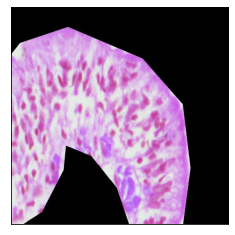}};
  \node[picture format,anchor=north]      (D1) at (C1.south) {\includegraphics[width=1.6in, height = 1.6in]{DeGPR/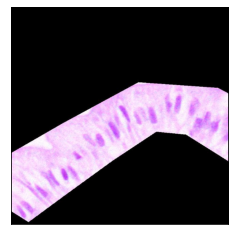}};
  
  \node[picture format,anchor=north west]                   (A2)   at (A1.north east)       {\includegraphics[width=1.6in, height = 1.6in]{DeGPR/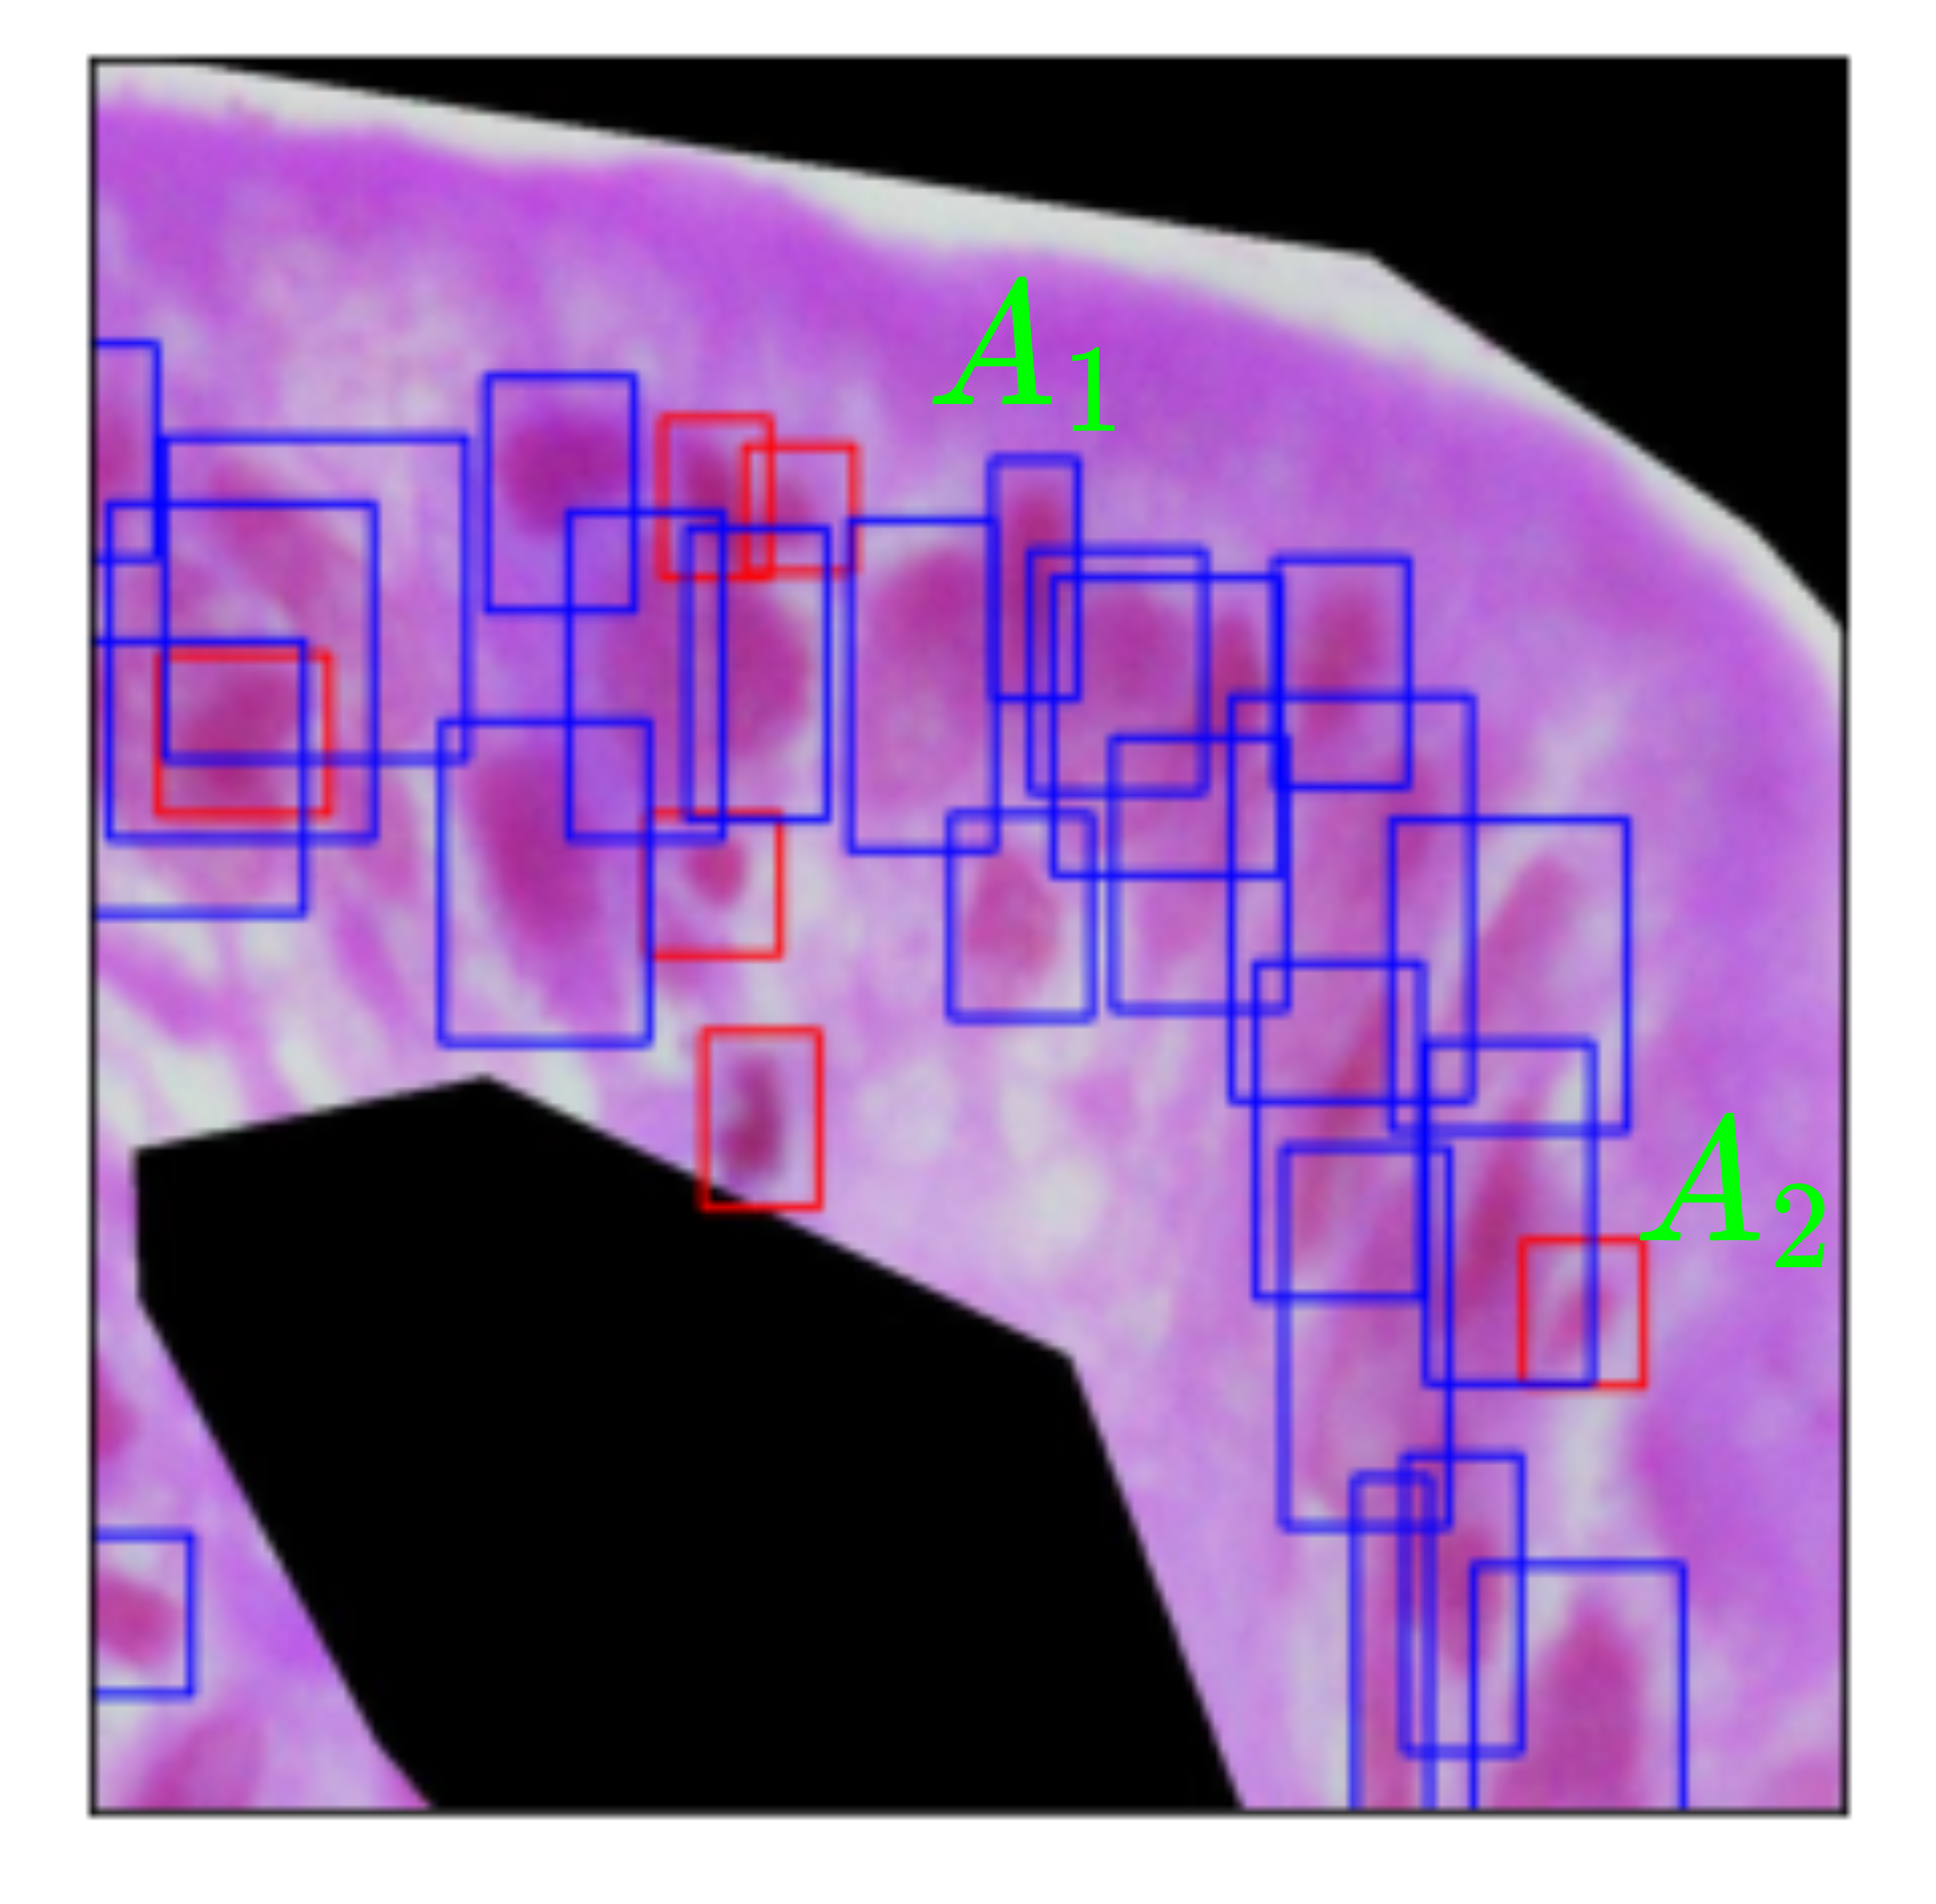}};
  \node[picture format,anchor=north]      (B2) at (A2.south) {\includegraphics[width=1.6in, height = 1.6in]{DeGPR/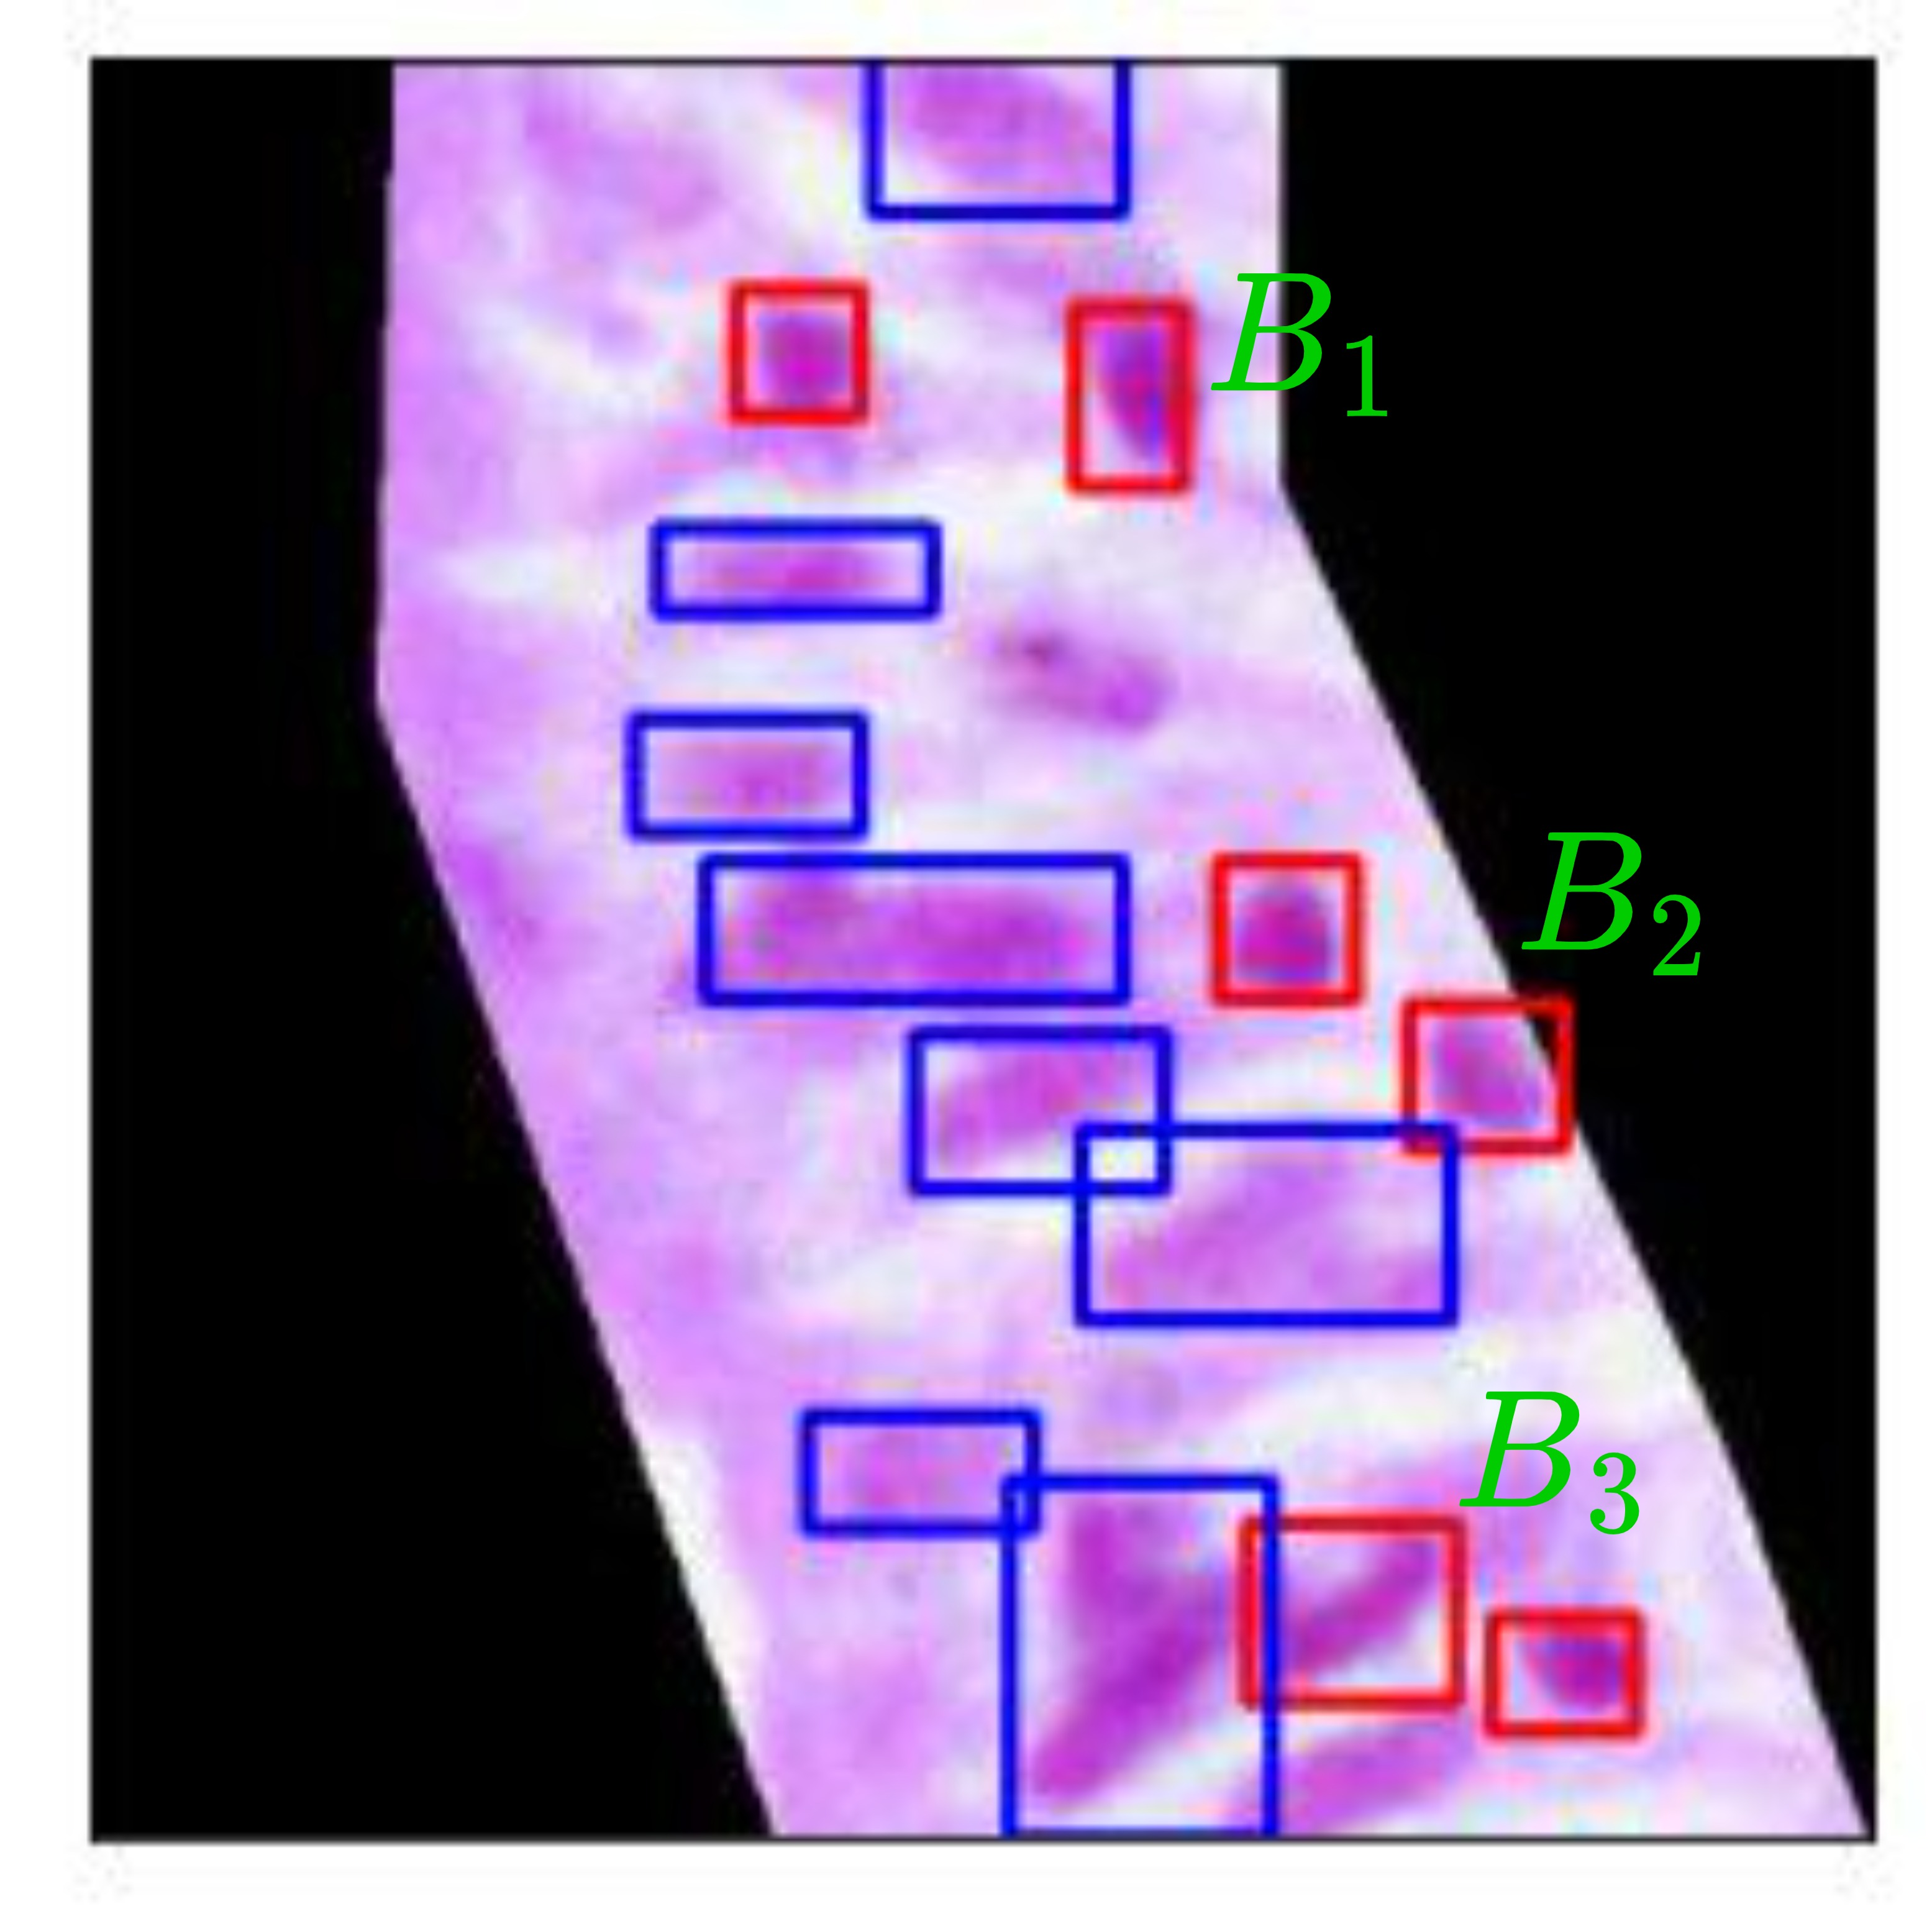}};
  \node[picture format,anchor=north]      (C2) at (B2.south) {\includegraphics[width=1.6in, height = 1.6in]{DeGPR/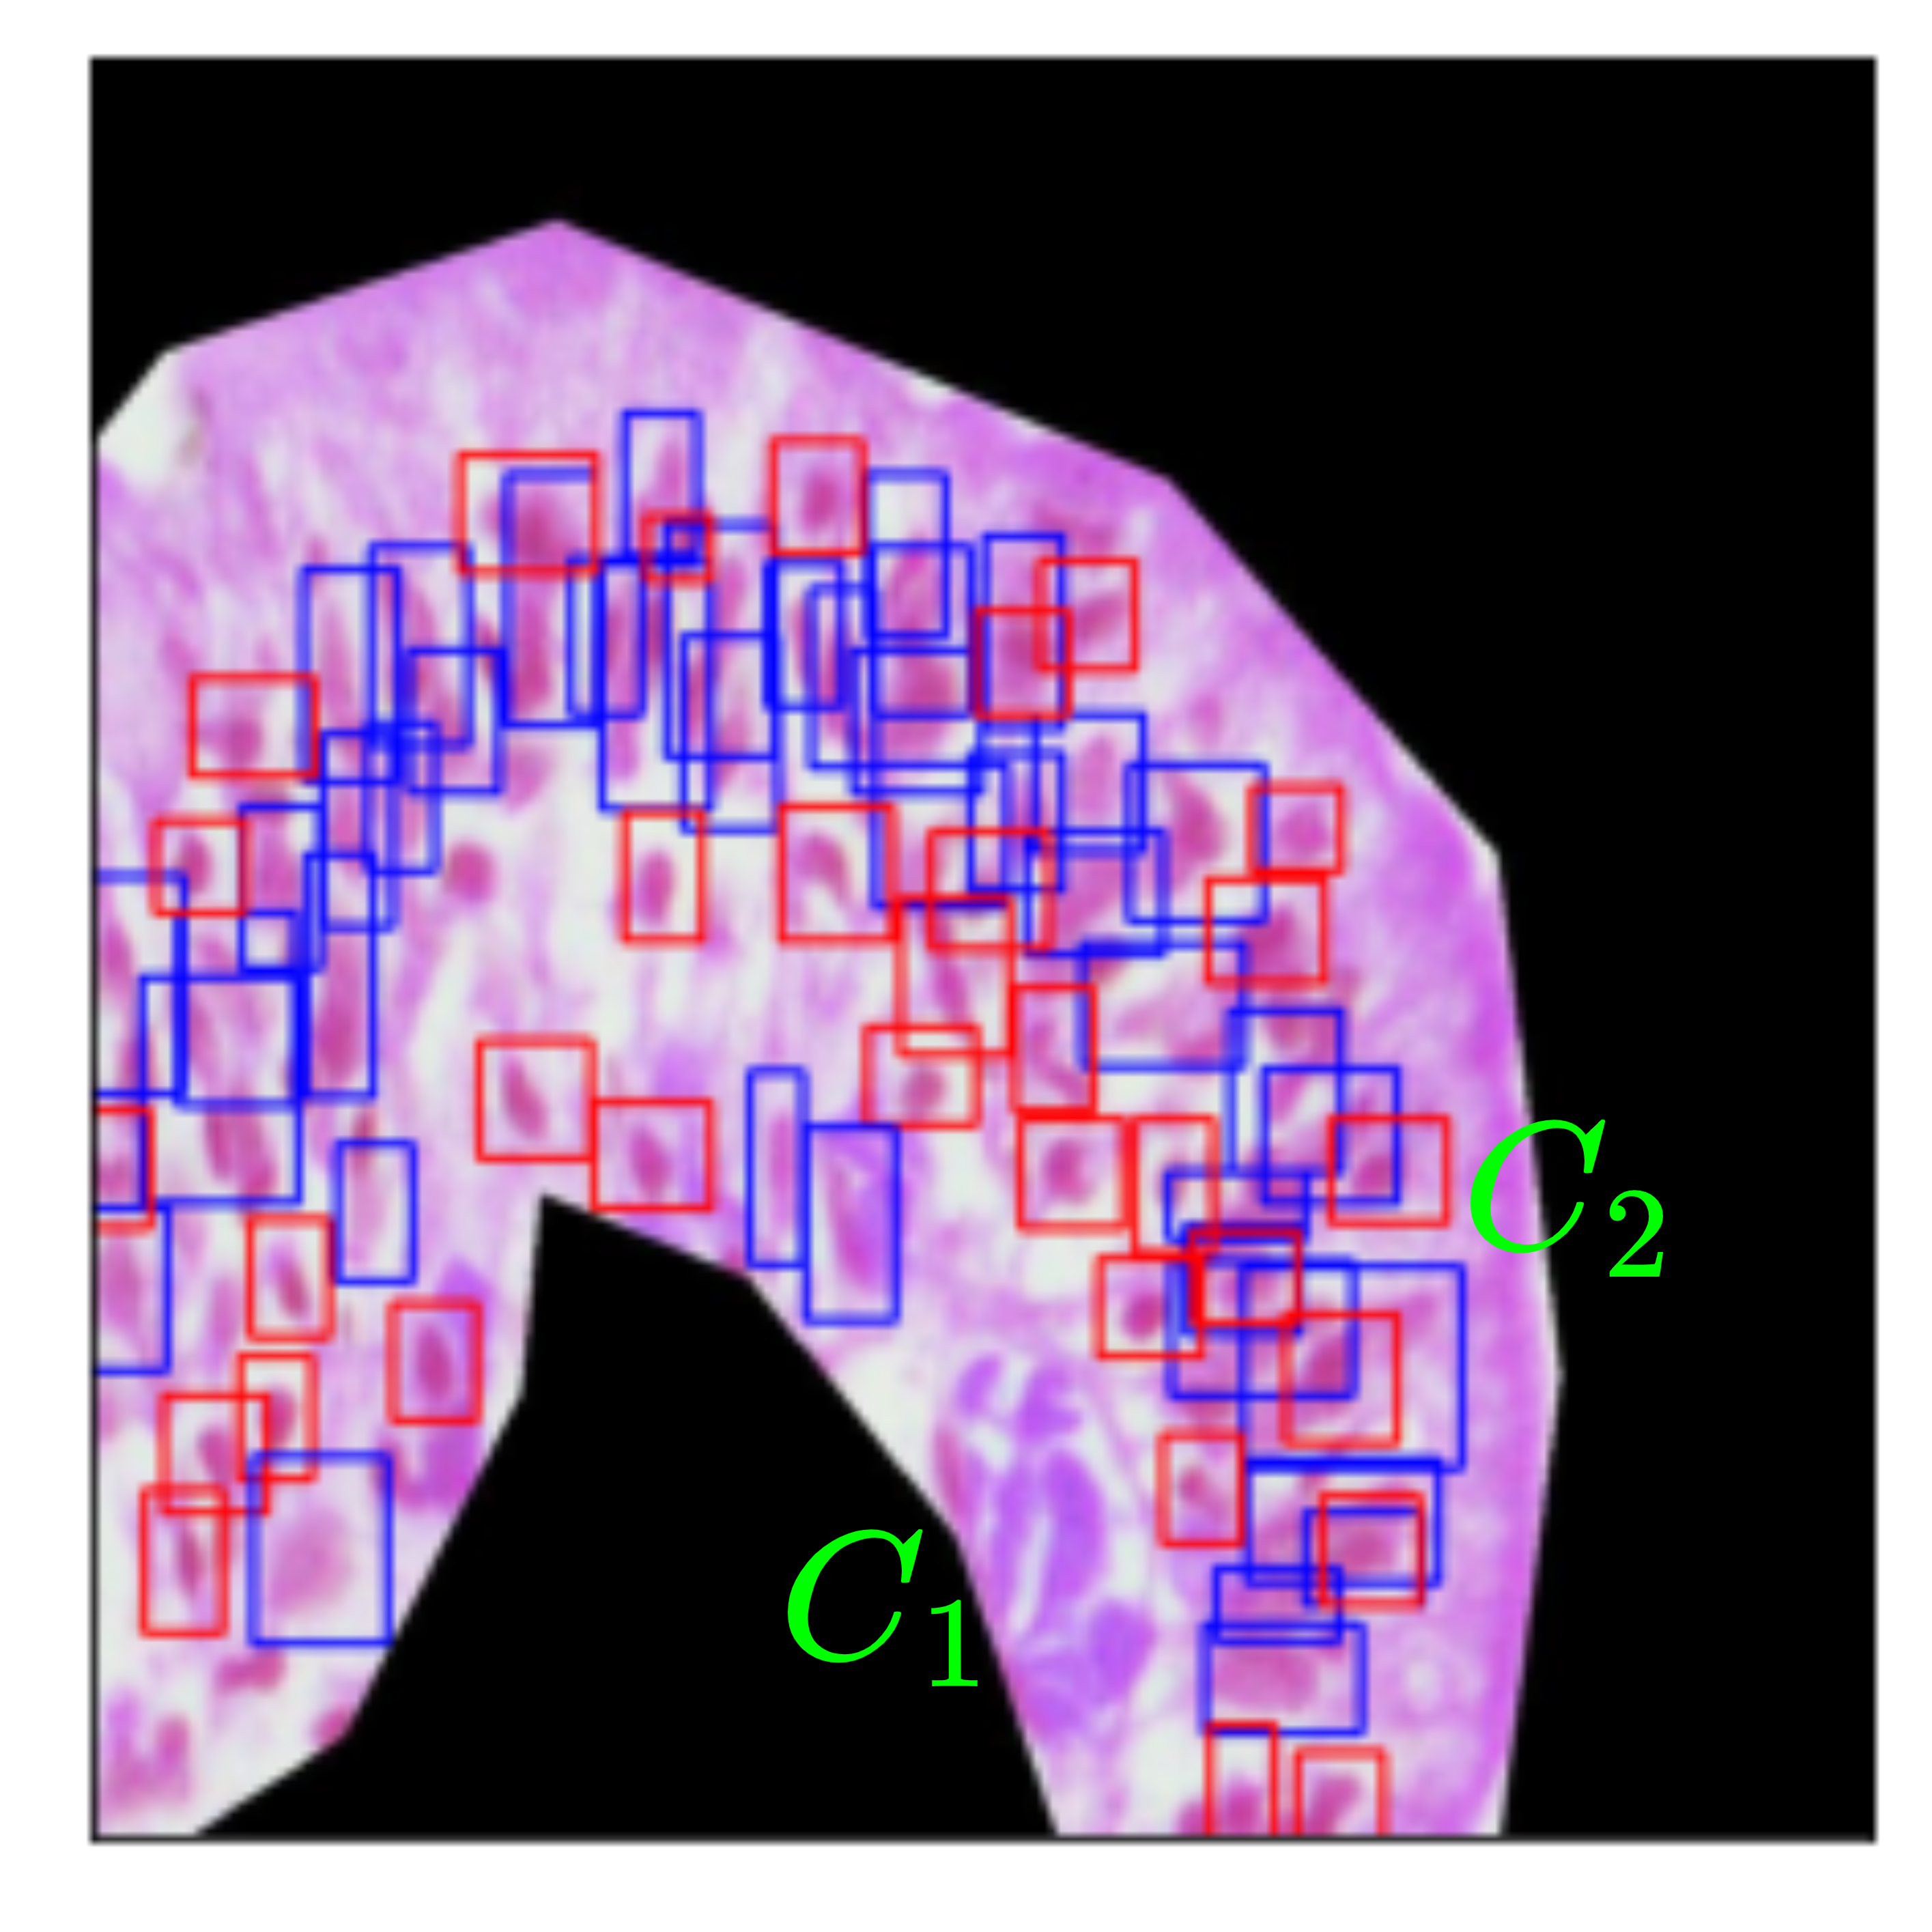}};
  \node[picture format,anchor=north]      (D2) at (C2.south) {\includegraphics[width=1.6in,  height = 1.6in]{DeGPR/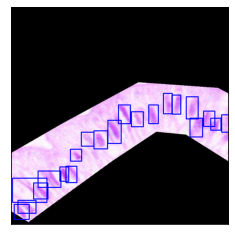}};

  \node[picture format,anchor=north west] (A3) at (A2.north east) {\includegraphics[width=1.6in, height = 1.6in]{DeGPR/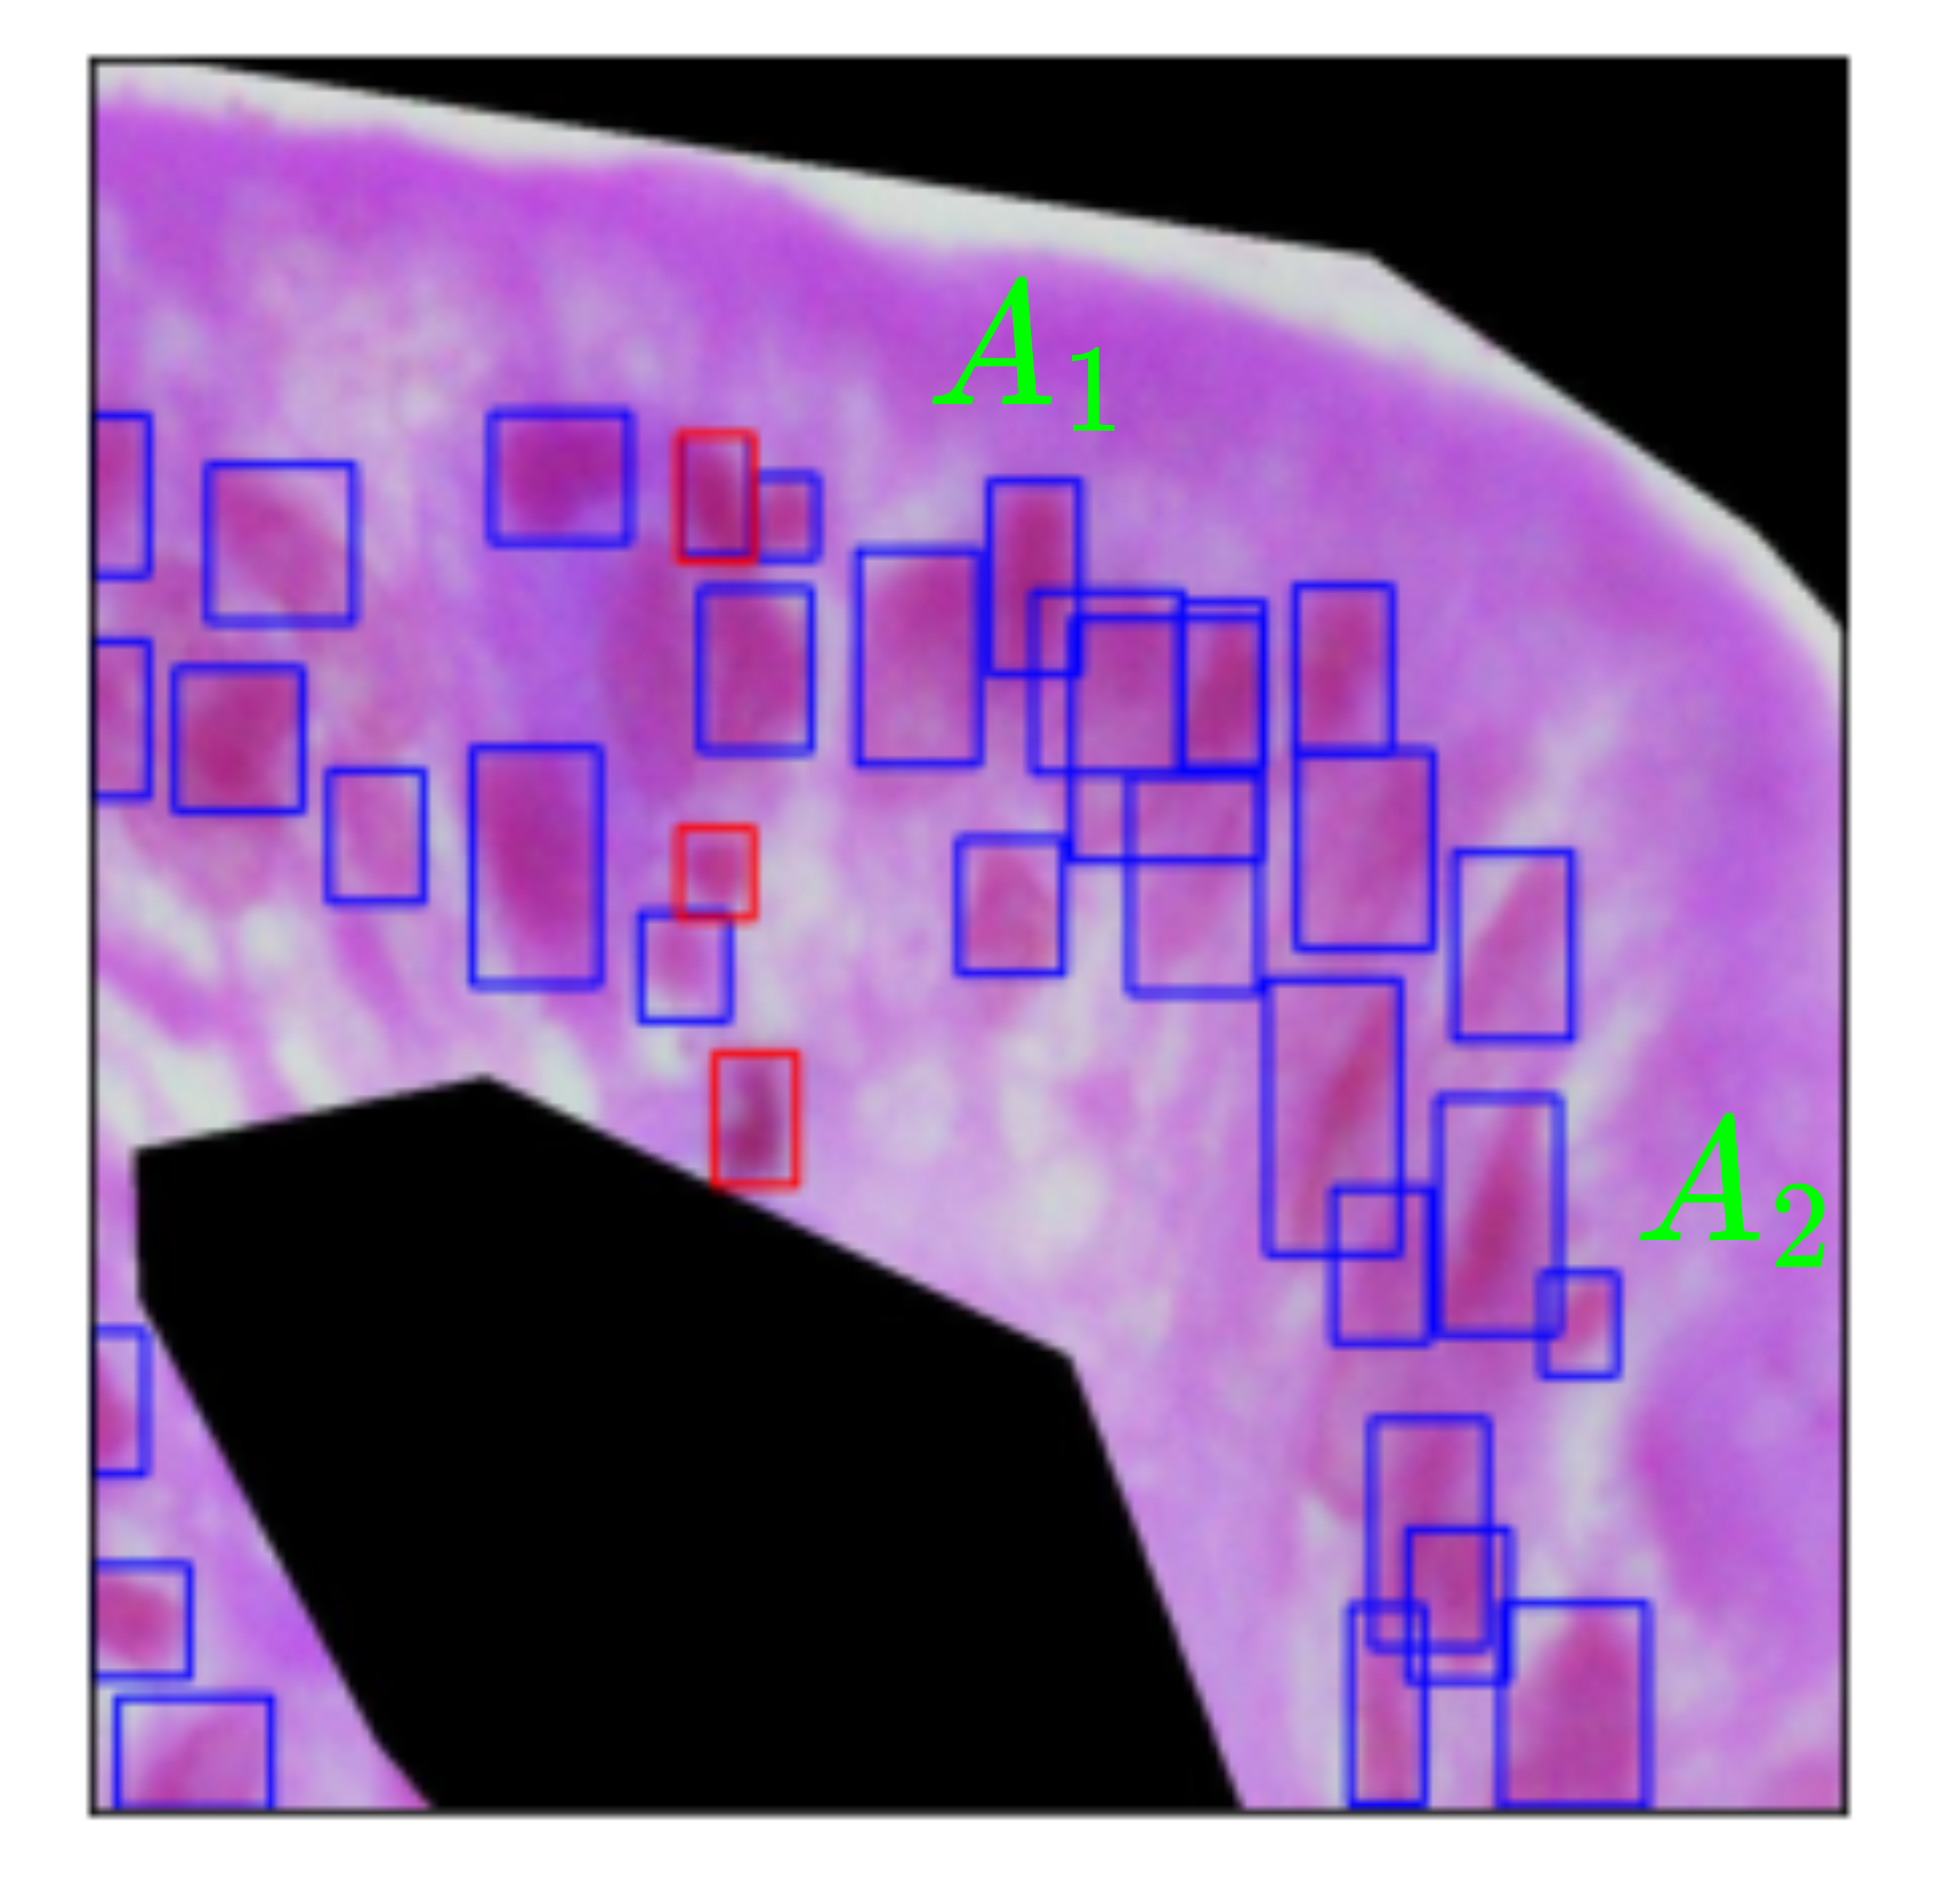}};
  \node[picture format,anchor=north]      (B3) at (A3.south)      {\includegraphics[width=1.6in, height = 1.6in]{DeGPR/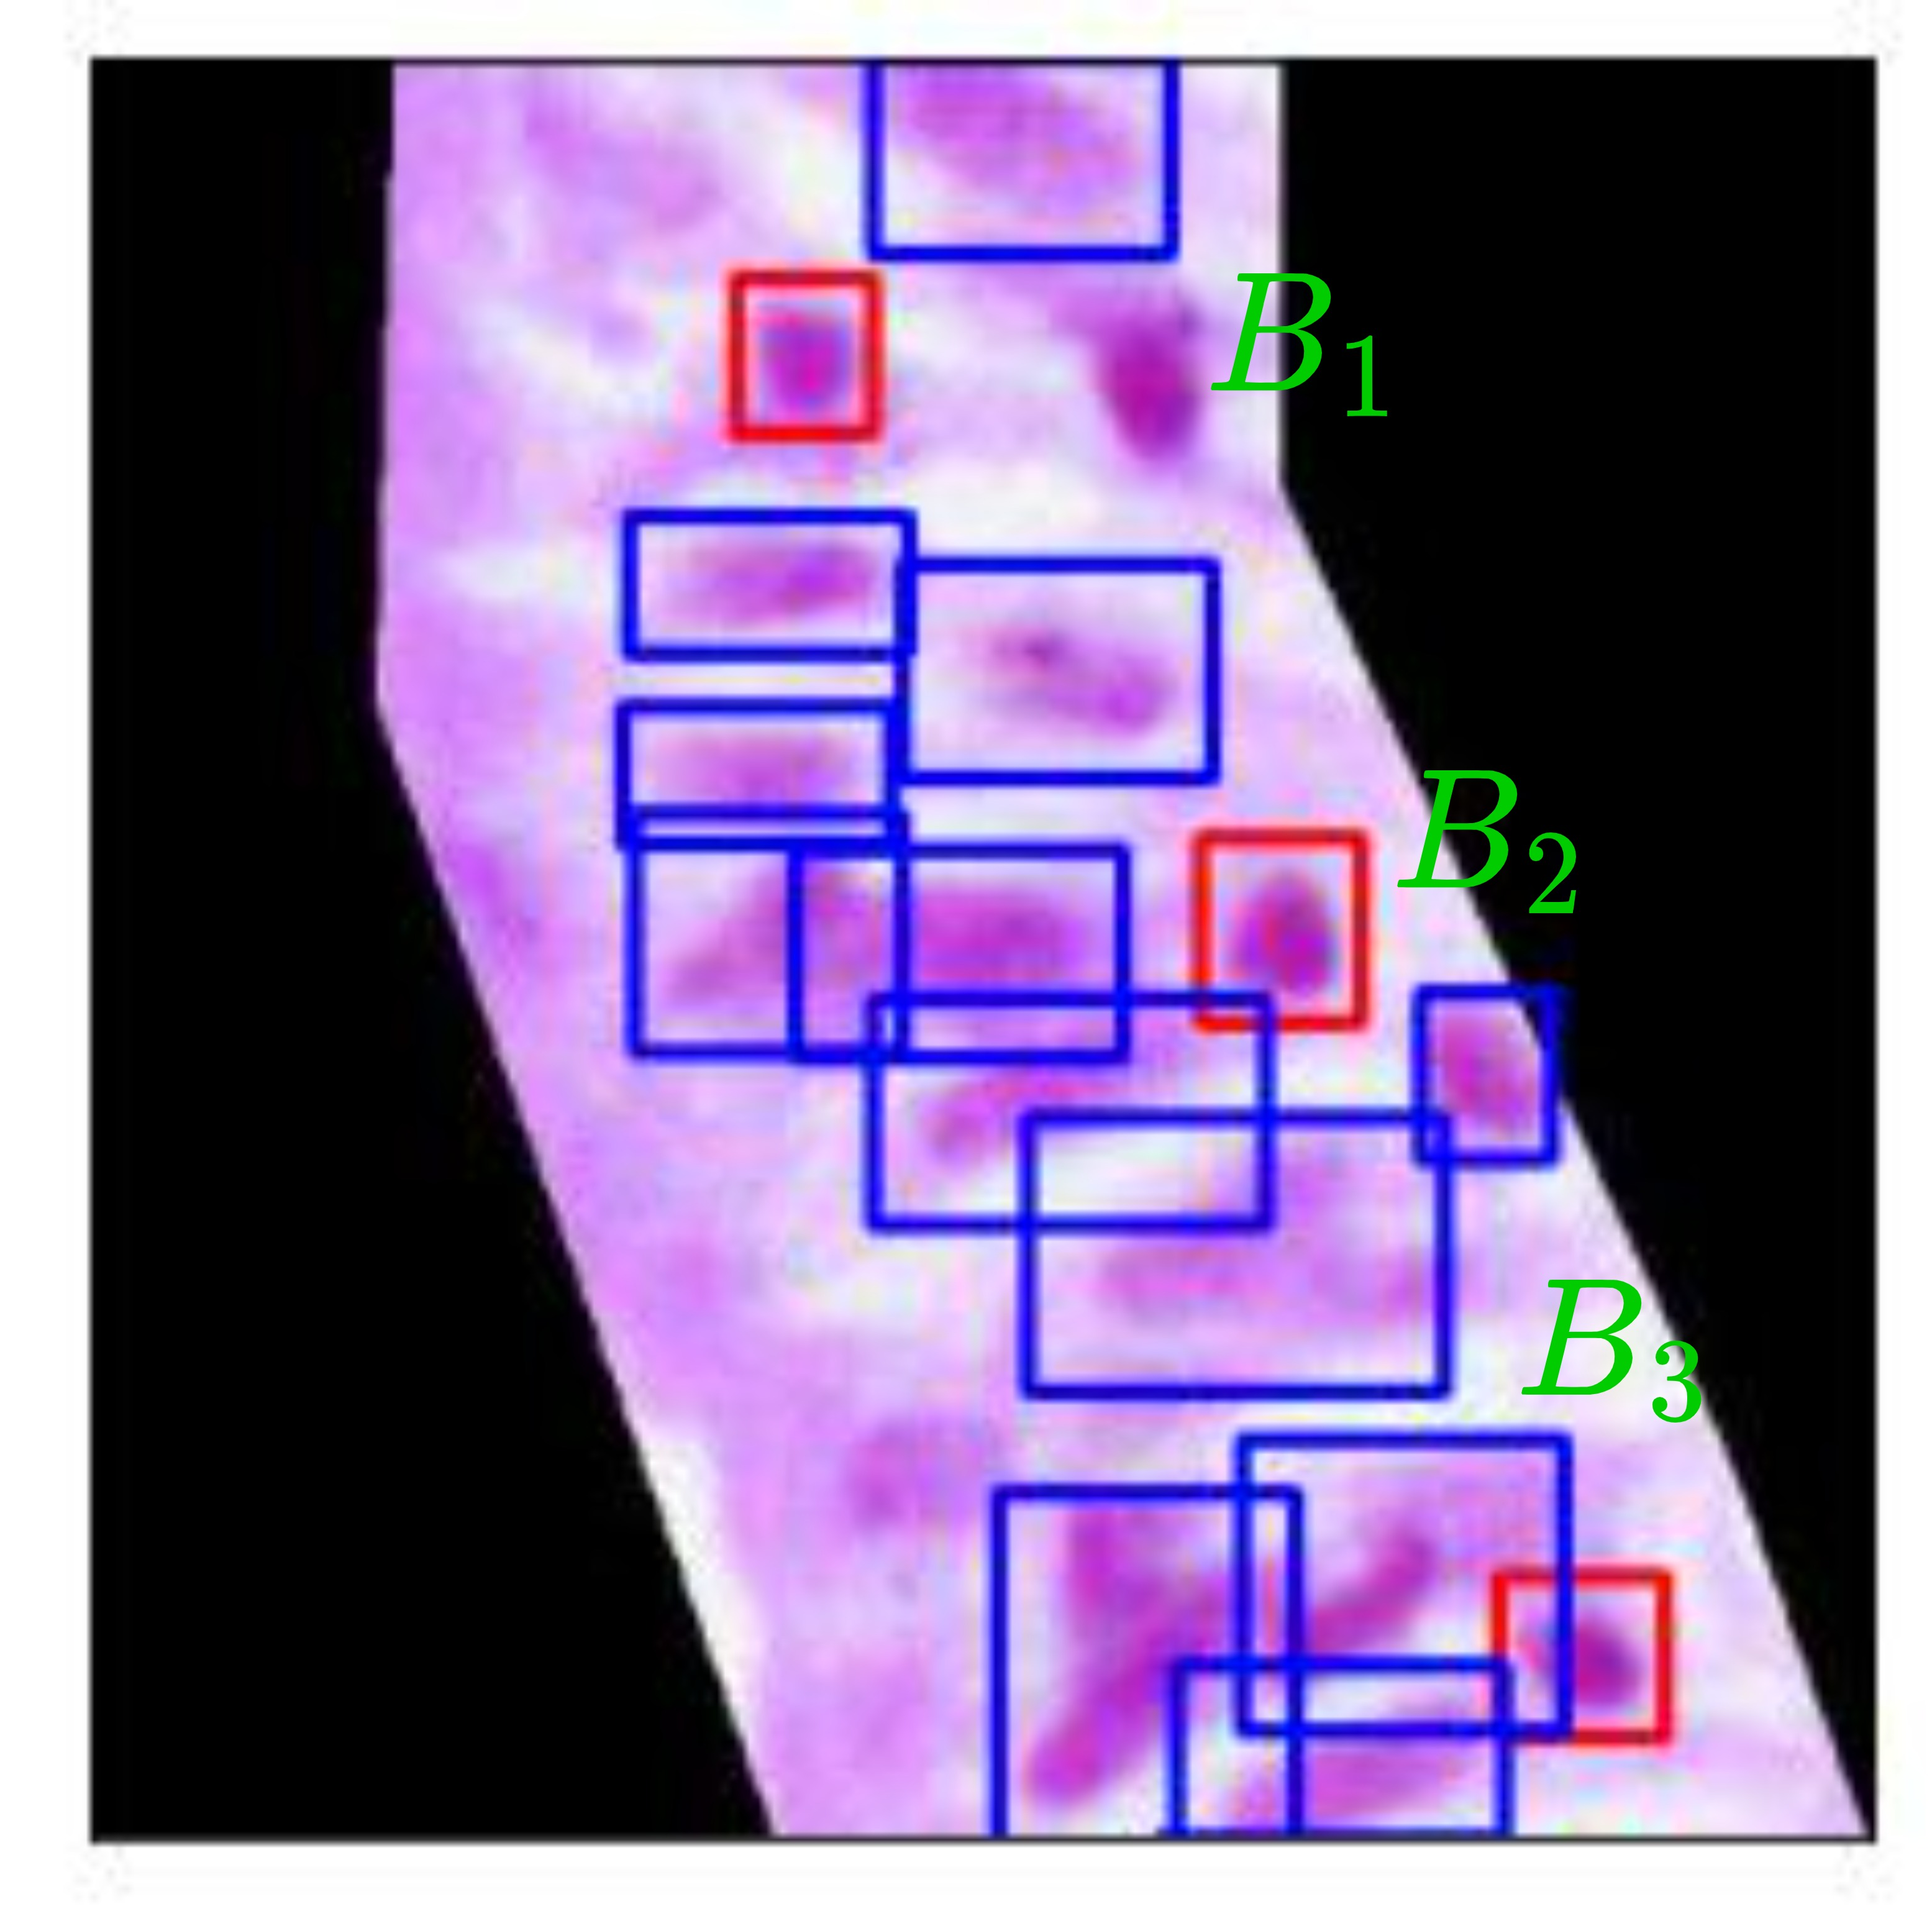}};
   \node[picture format,anchor=north]      (C3) at (B3.south)      {\includegraphics[width=1.6in, height=1.6in]{DeGPR/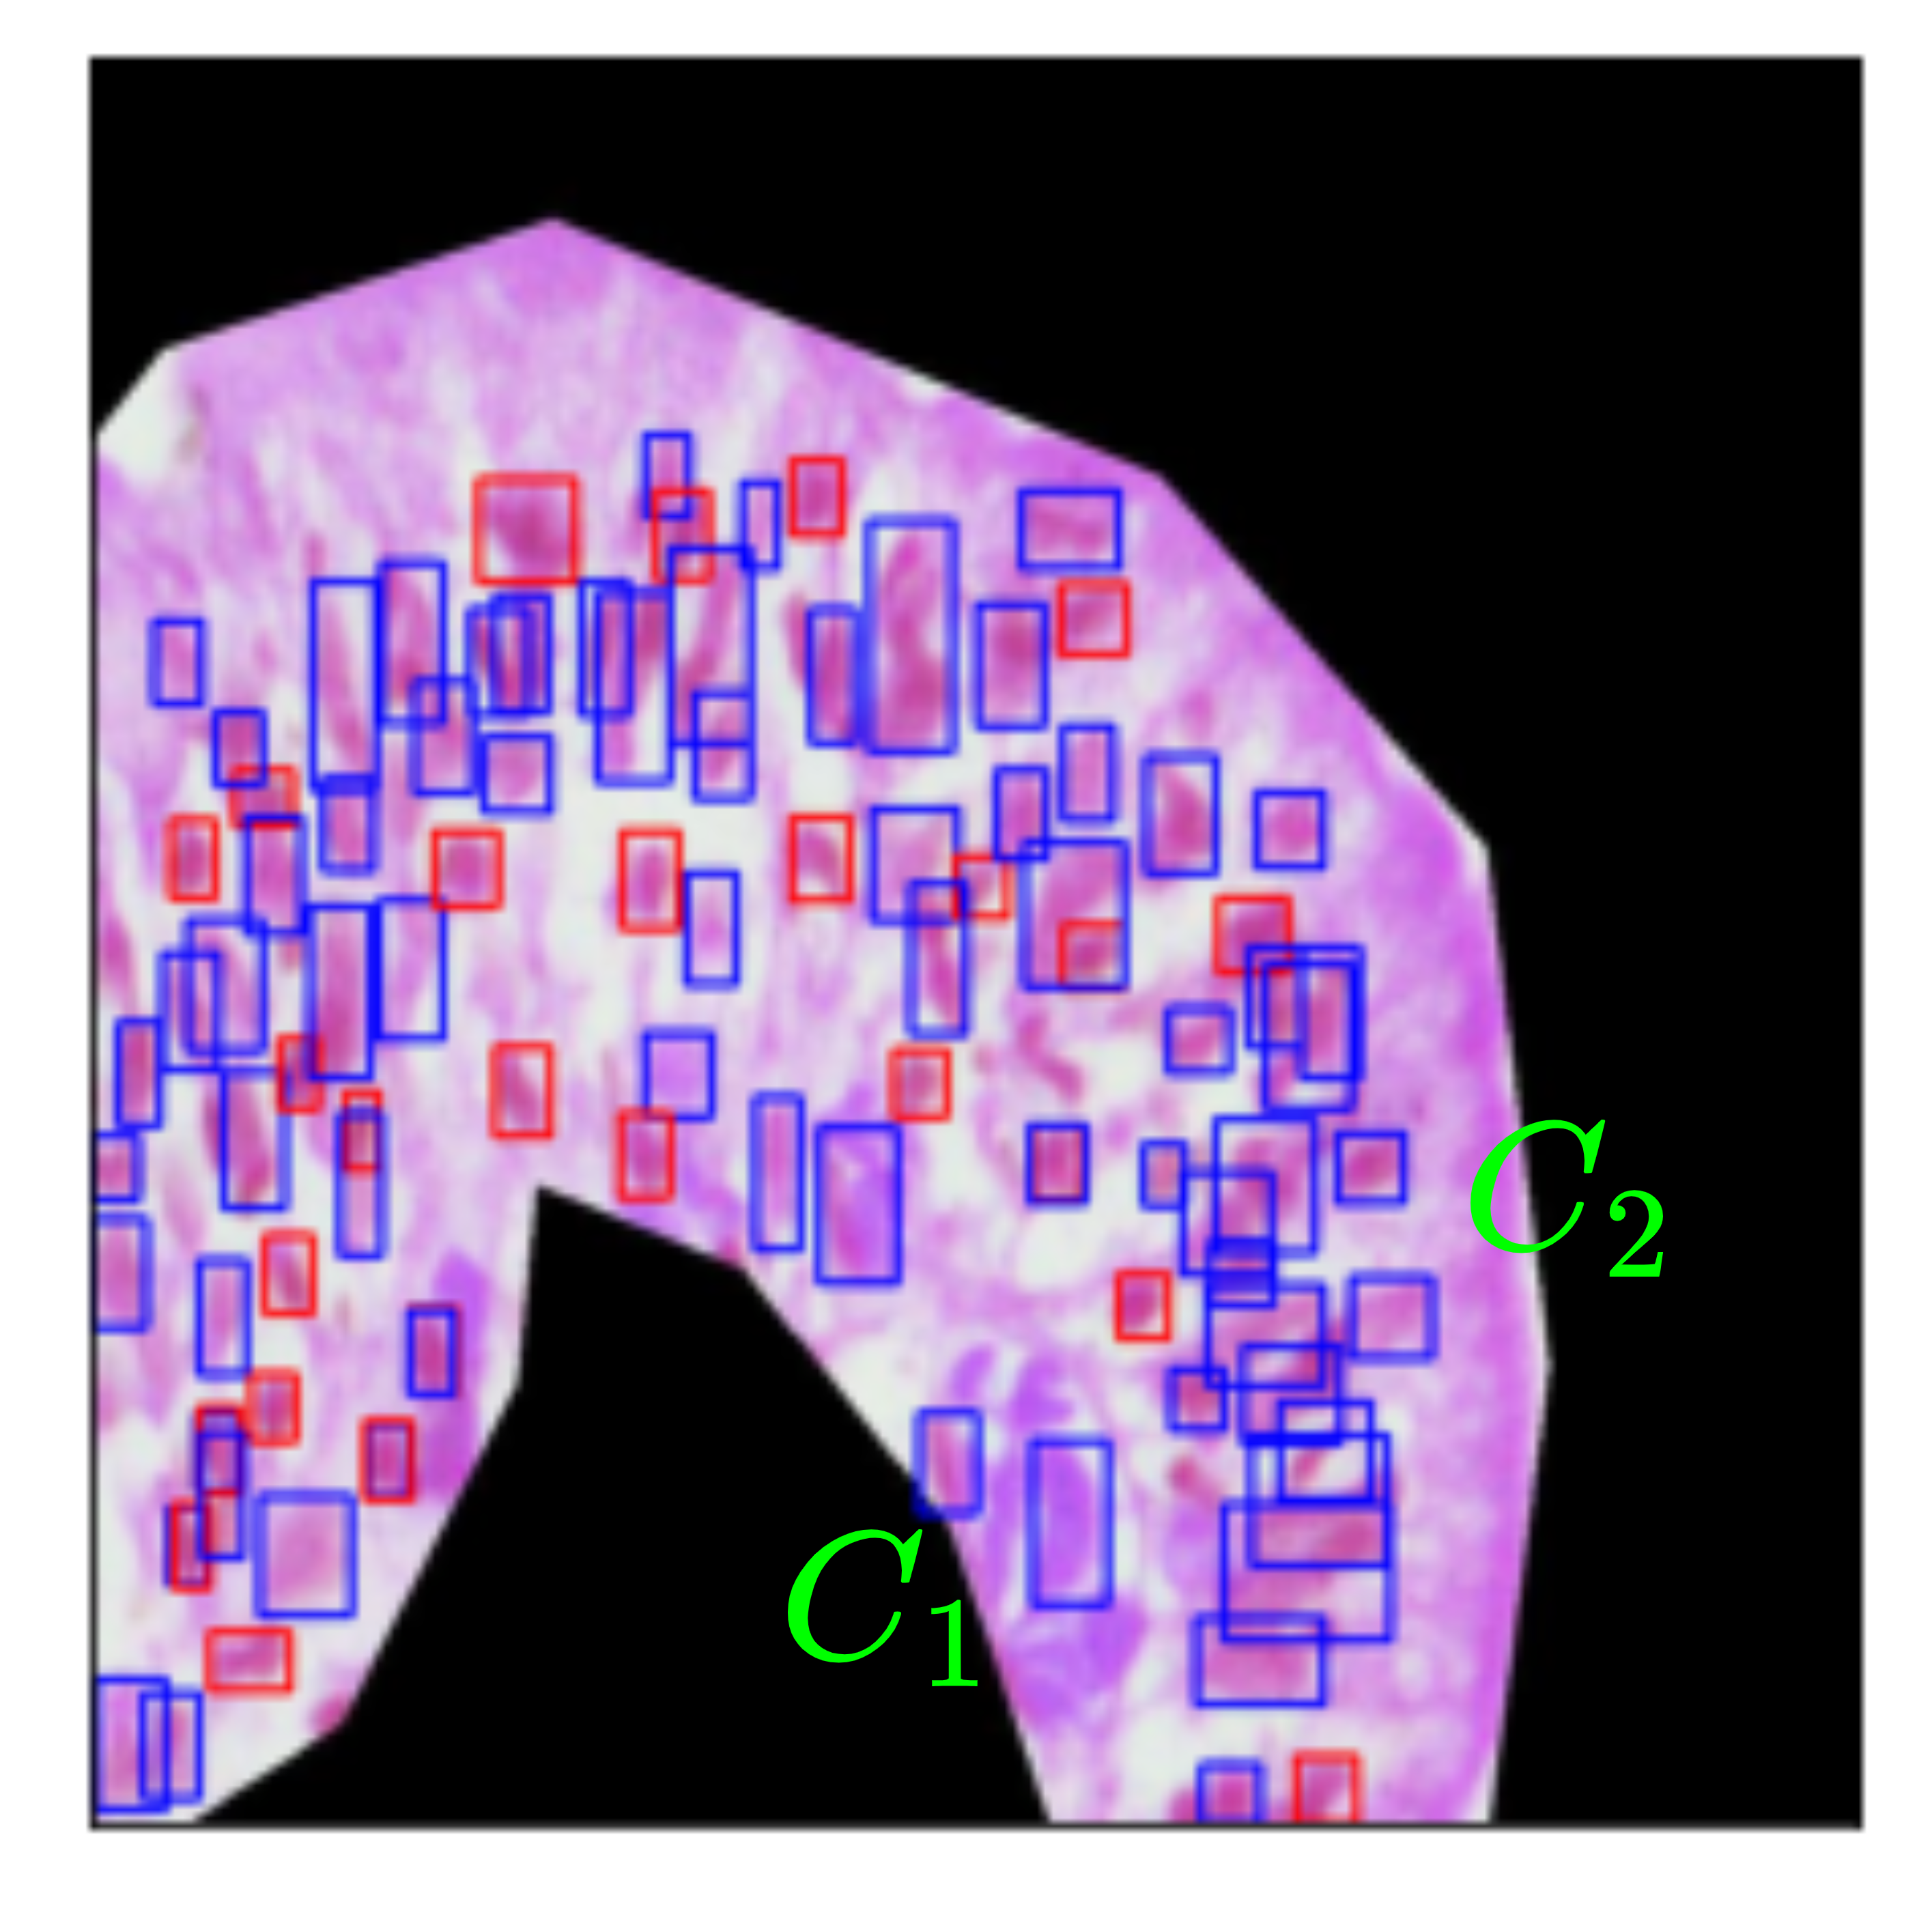}};
   \node[picture format,anchor=north]      (D3) at (C3.south)      {\includegraphics[width=1.6in, height = 1.6in]{DeGPR/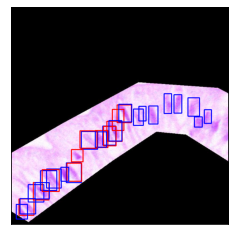}};

  \node[picture format,anchor=north west] (A4) at (A3.north east) {\includegraphics[width=1.6in, height = 1.6in]{DeGPR/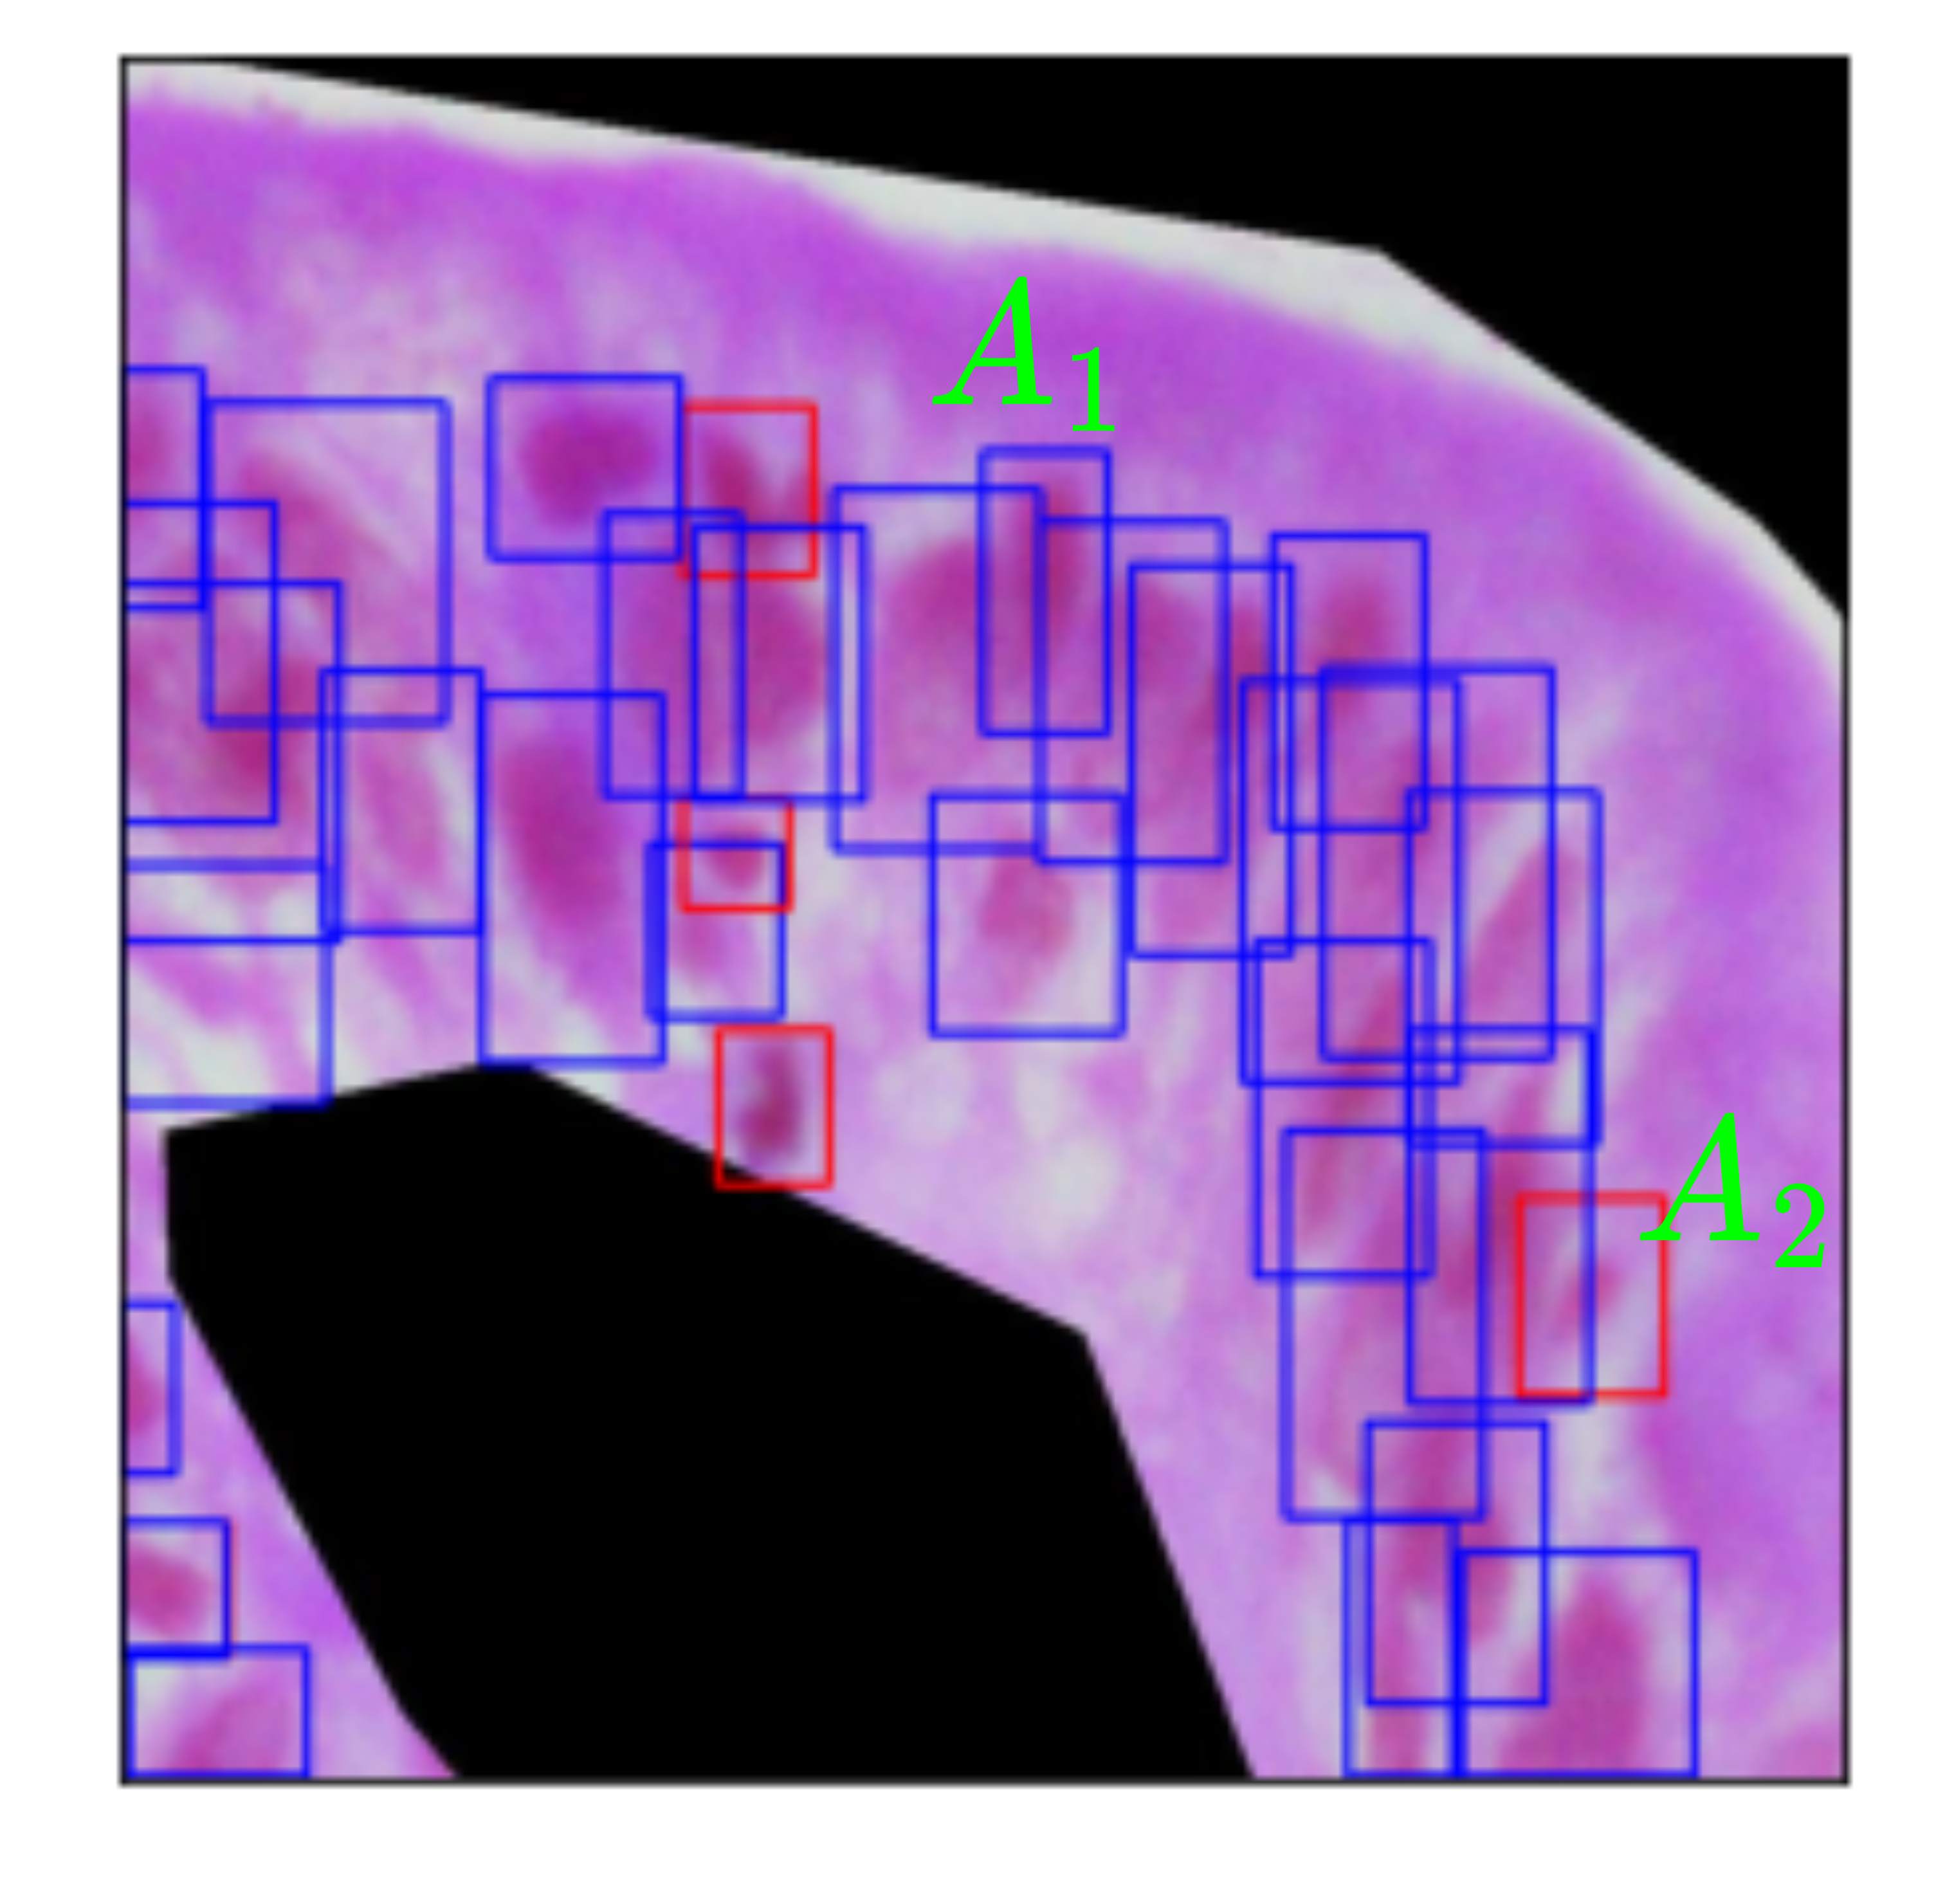}};
  \node[picture format,anchor=north]      (B4) at (A4.south)      {\includegraphics[width=1.6in, height = 1.6in]{DeGPR/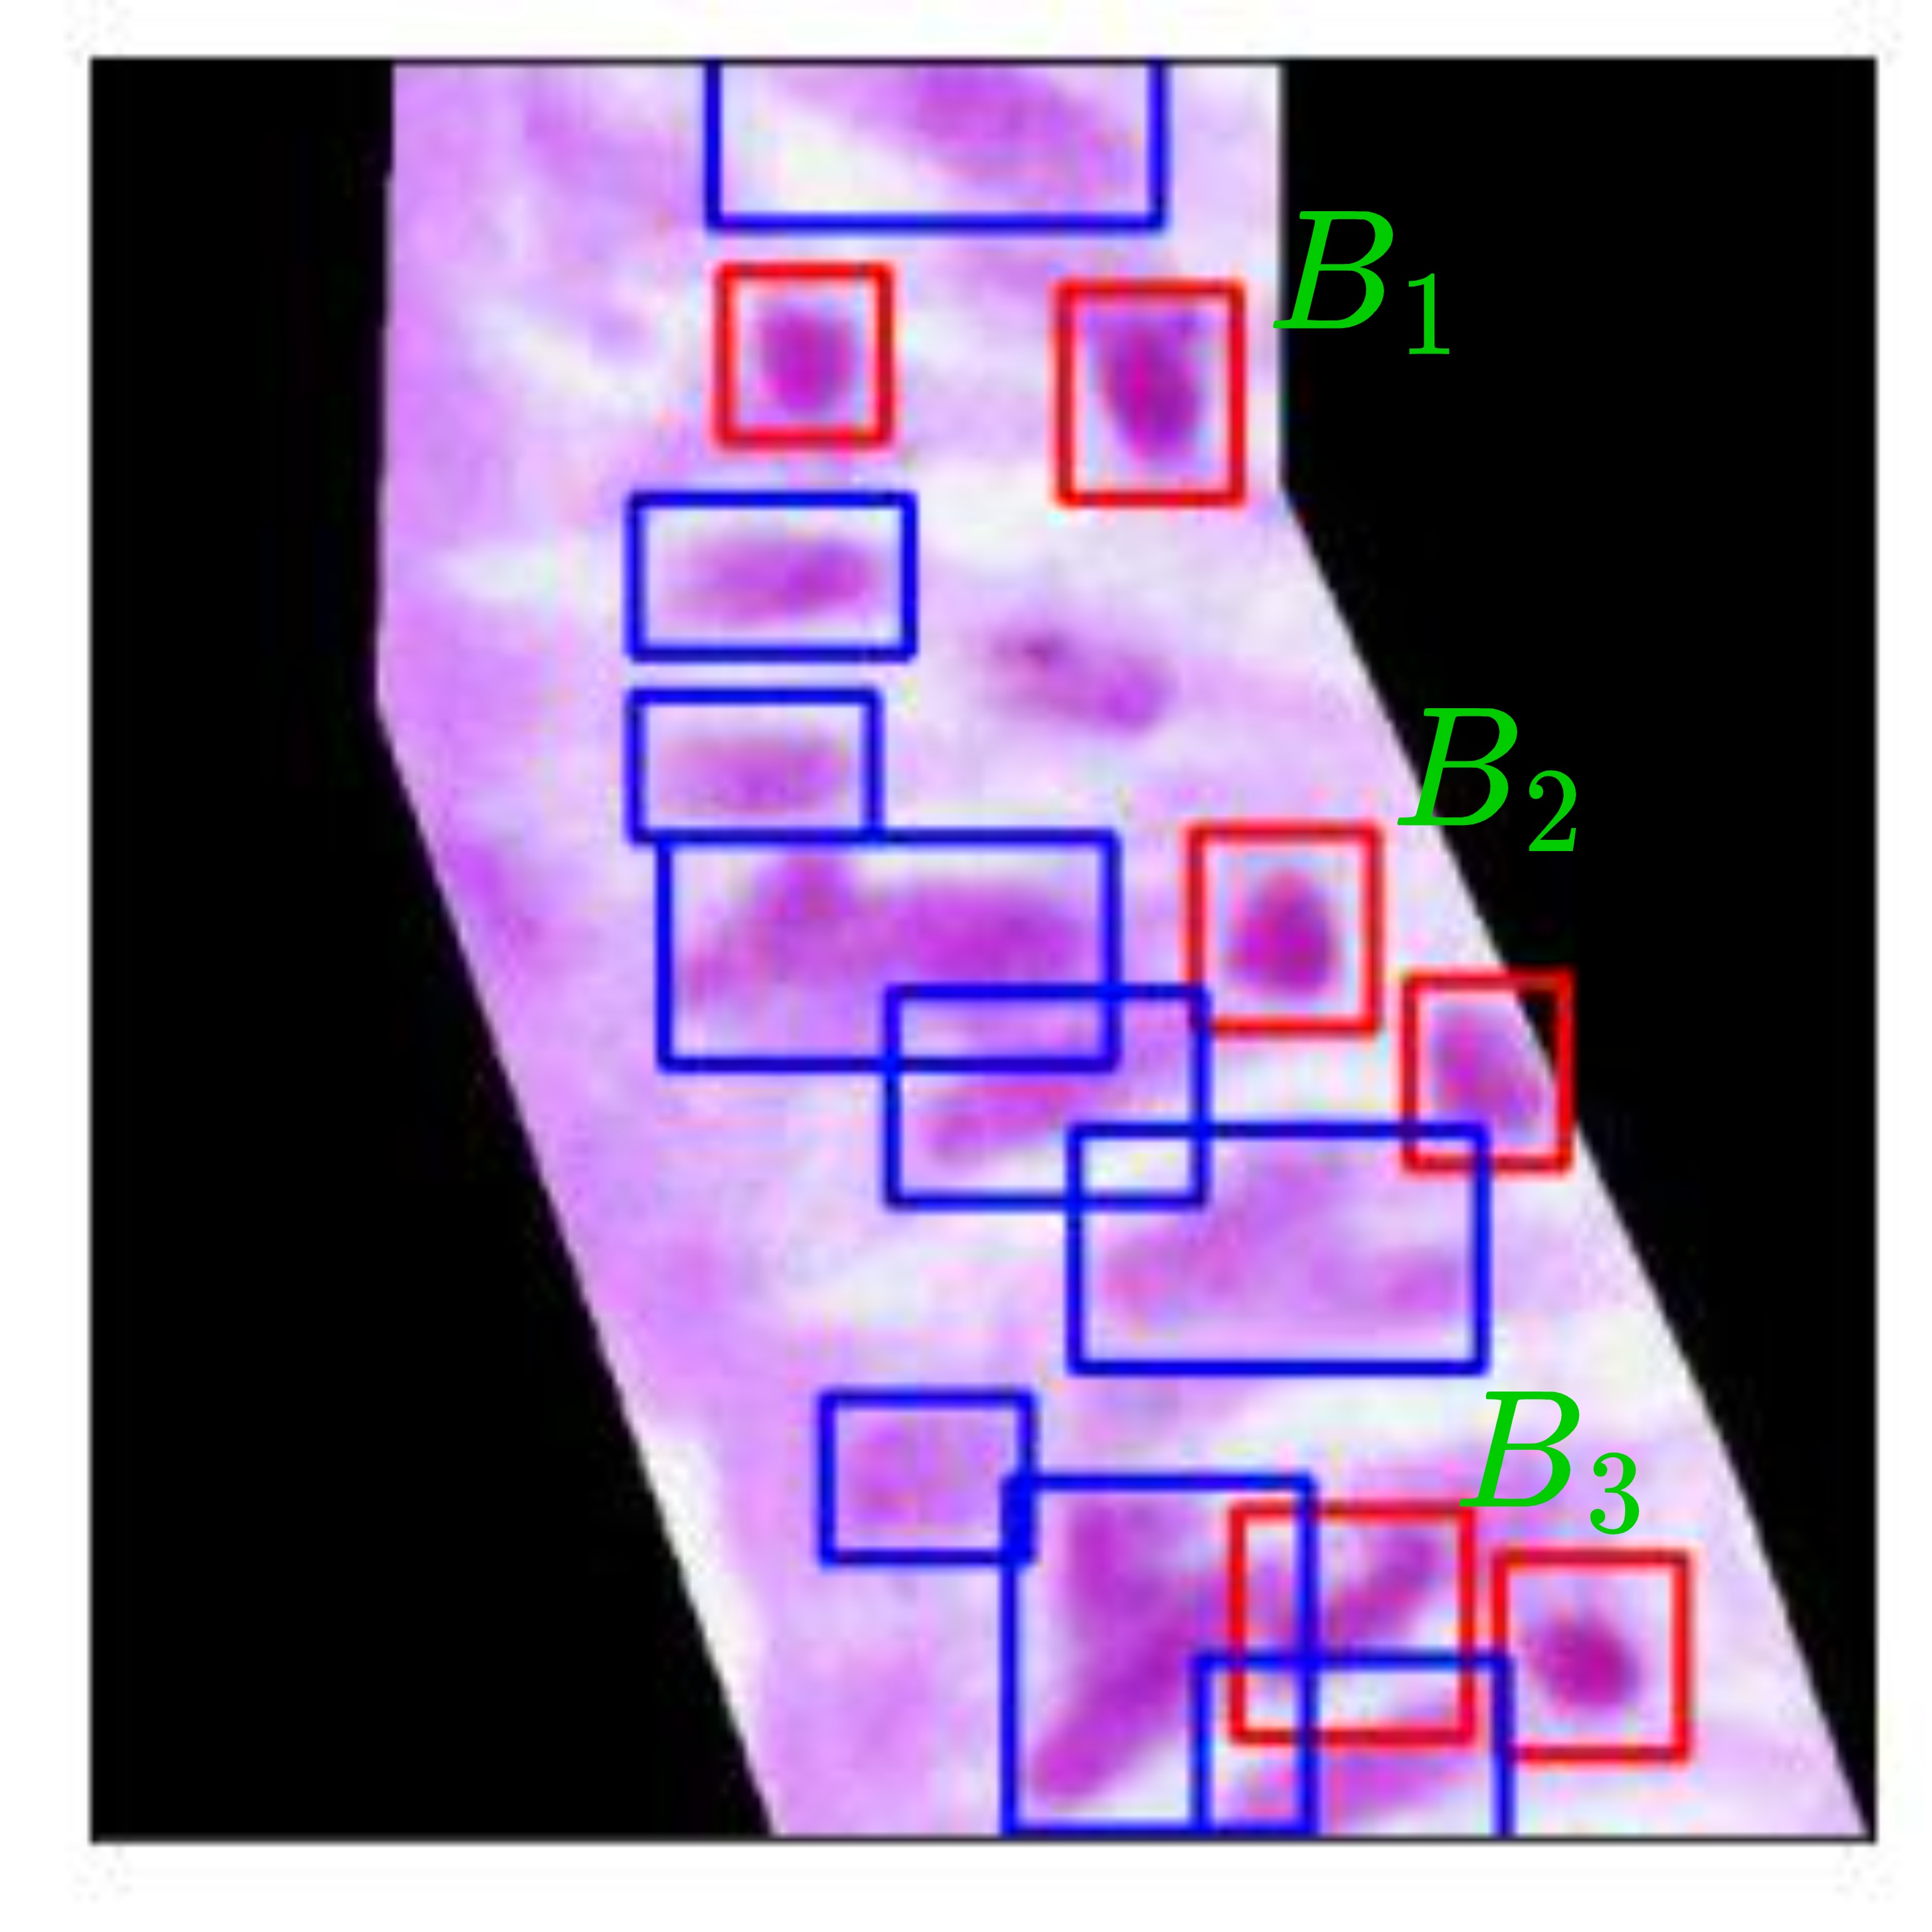}};
  \node[picture format,anchor=north]      (C4) at (B4.south)      {\includegraphics[width=1.6in, height=1.6in]{DeGPR/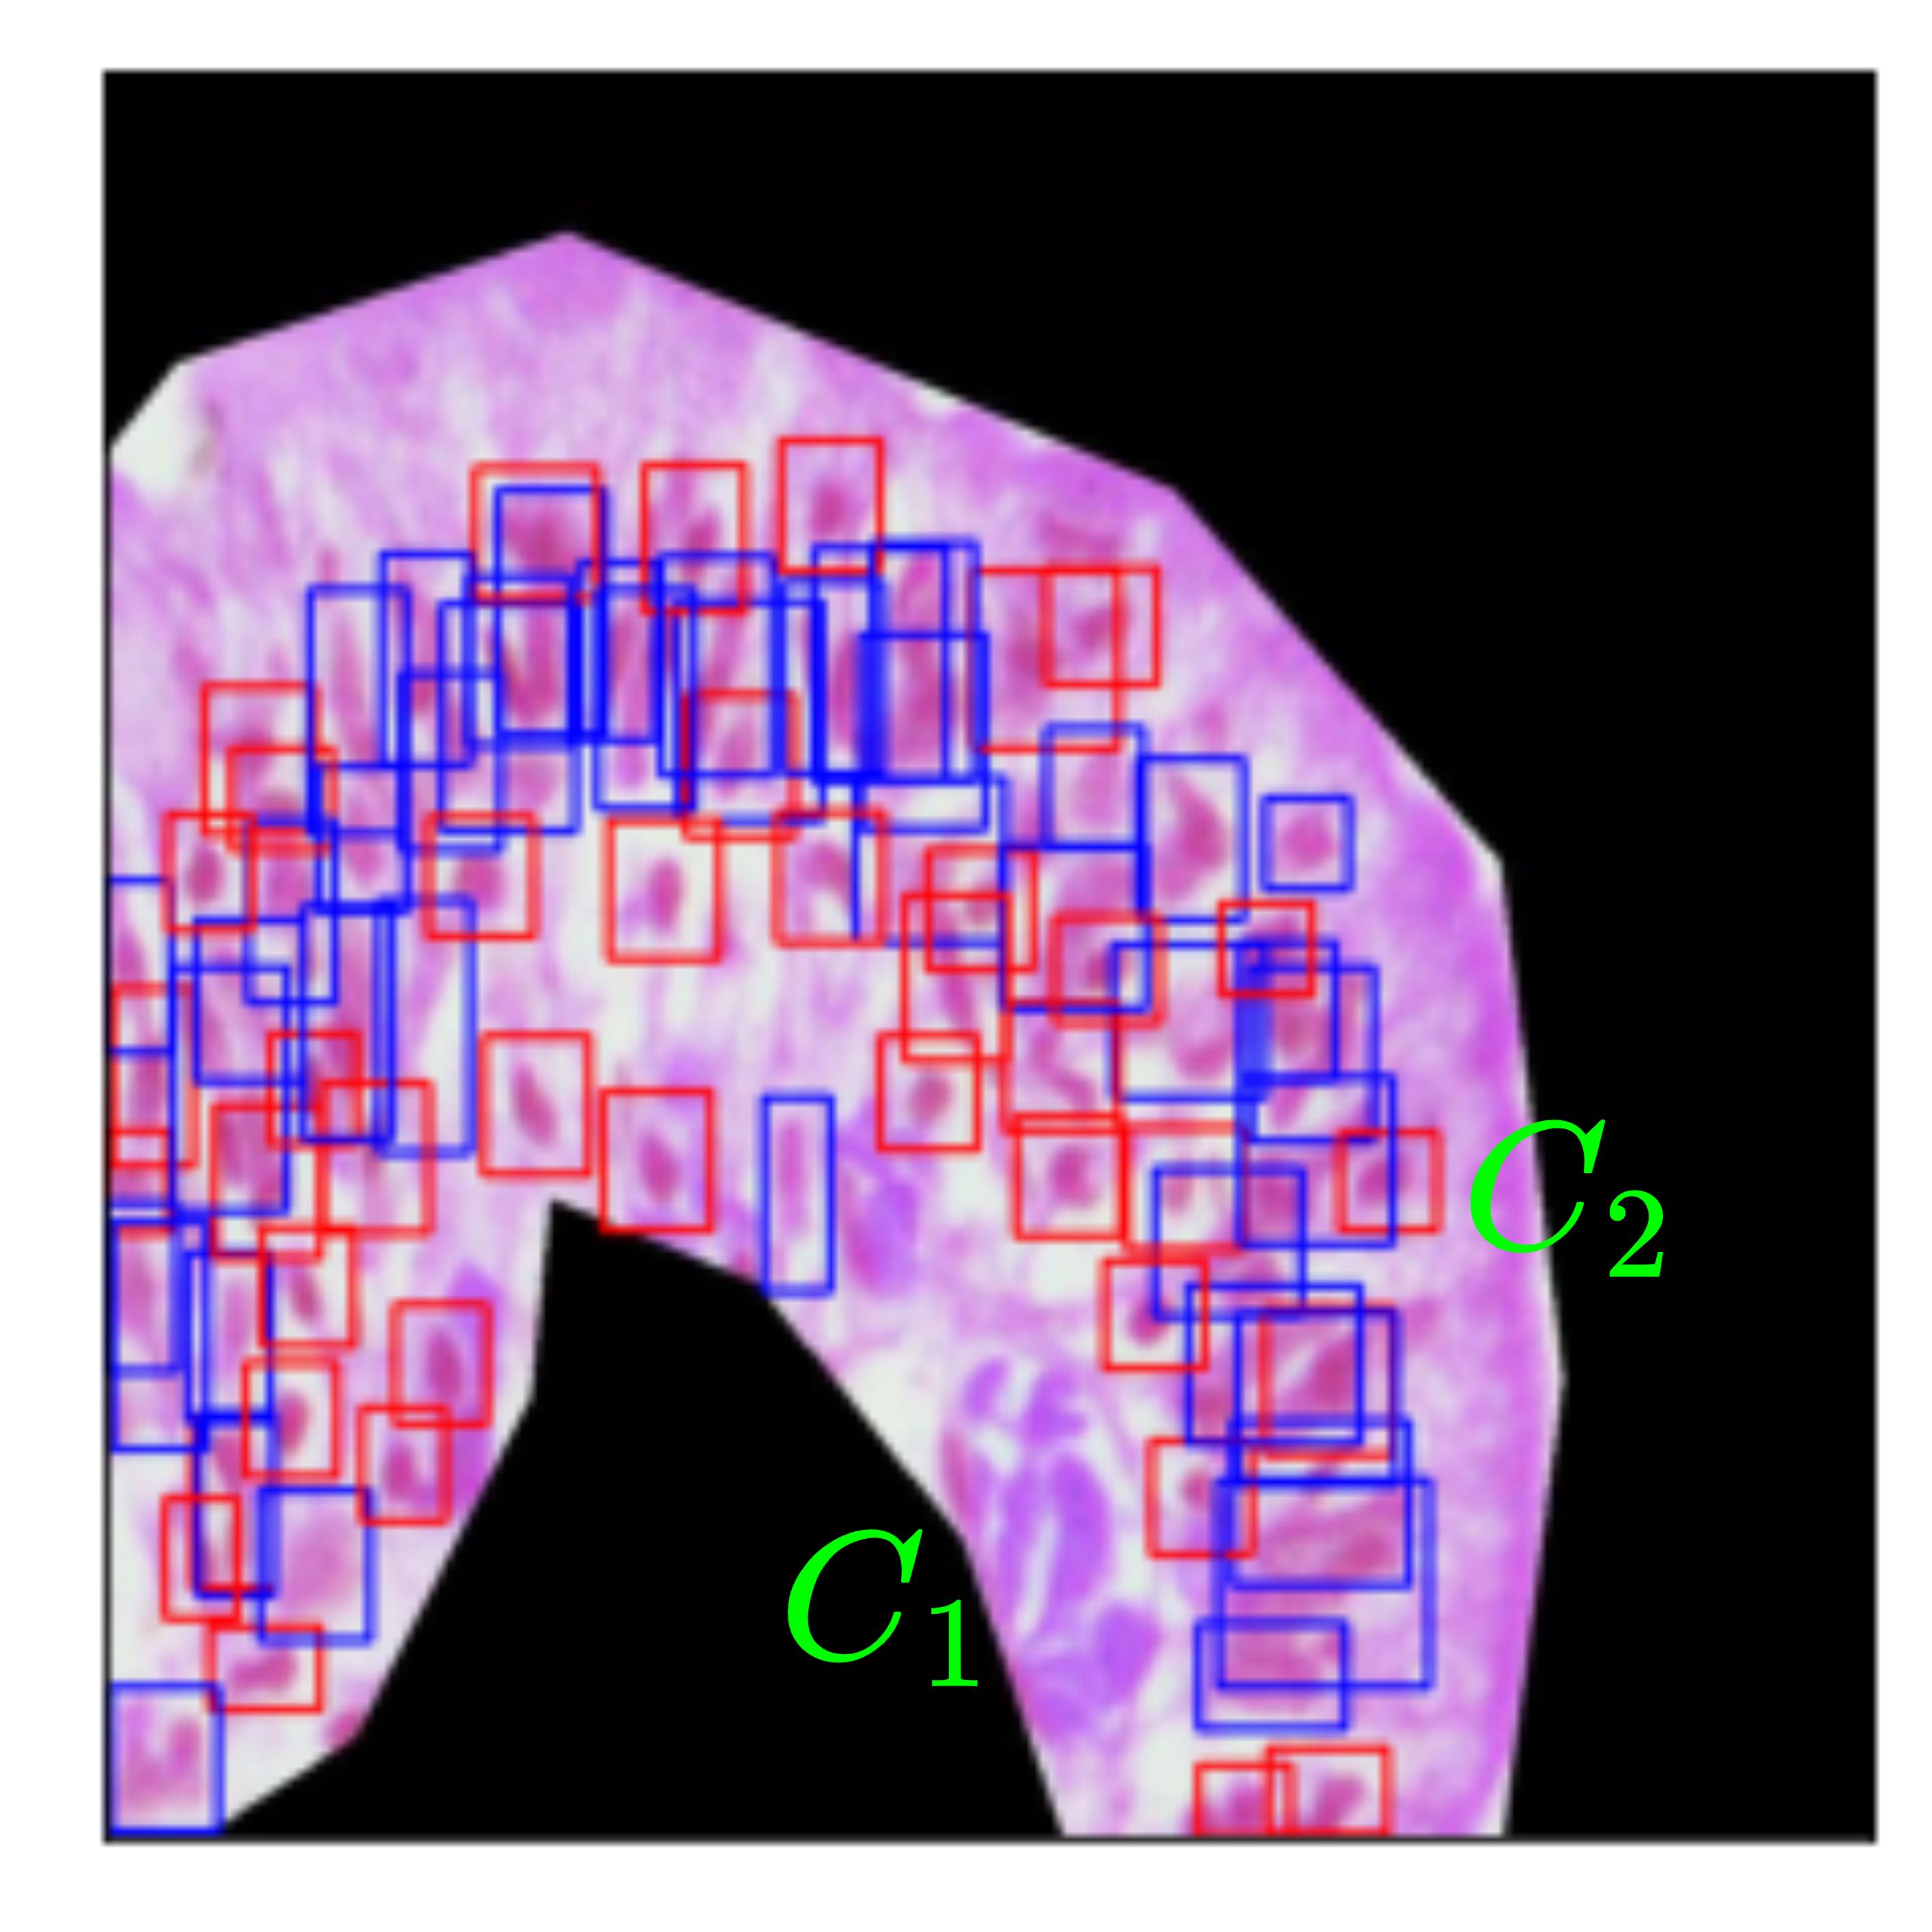}};
  \node[picture format,anchor=north]      (D4) at (C4.south)      {\includegraphics[width=1.6in, height = 1.6in]{DeGPR/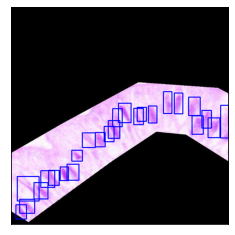}};
  %% Captions

  \node[anchor=south] (C1) at (A1.north) {\bfseries Original};
  \node[anchor=south] (C2) at (A2.north) {\bfseries Ground Truth};
  \node[anchor=south] (C3) at (A3.north) {\bfseries Baseline};
  \node[anchor=south] (C4) at (A4.north) {\bfseries Proposed};

\end{tikzpicture}
\caption{Qualitative performance of \sys{} for MuCeD. The cells are marked as Blue (EN) and Red(IEL). In the first row, in the region $A_1$, we can see that the baseline model misses multiple Epithelial Nuclei which are overlapping. The model with \sys{} performs better here. In region $A_2$, the baseline model misclassifies an IEL as an EN. In the second row, the regions $B_1,B_2,B_3$ show reduction in misclassfication errors as well as cells which were missed. In the third row, in region $C_1$, the baseline model makes extra predictions which the model with \sys{} has solved. In region $C_2$, there is an IEL which is inside an EN(in 3-d, it is on top of the EN). The model with \sys{} is successfully able to detect the IEL. Finally, the fourth row has cells of very light intensity. While the baseline model makes misclassifications, the model with \sys{} is successful in detecting all cells correctly.}
\label{fig: bbox_prediction_MuCeD_sup}
\end{figure*}

\begin{figure*}
\centering
\begin{tikzpicture}[scale=1.03,transform shape, picture format/.style={inner sep=1pt}]

  \node[picture format]                   (A1)   at (0,0)            {\includegraphics[width=1.6in, height = 1.6in]{DeGPR/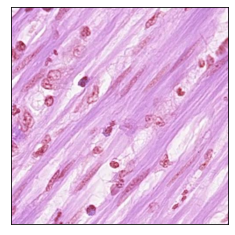}};
  \node[picture format,anchor=north]      (B1) at (A1.south) {\includegraphics[width=1.6in, height = 1.6in]{DeGPR/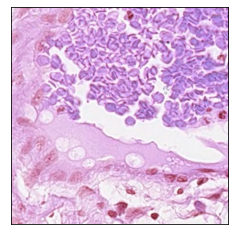}};
  \node[picture format,anchor=north]      (C1) at (B1.south) {\includegraphics[width=1.6in, height = 1.6in]{DeGPR/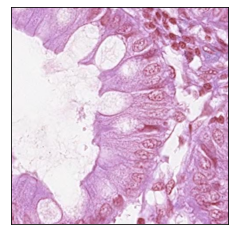}};
  \node[picture format,anchor=north]      (D1) at (C1.south) {\includegraphics[width=1.6in, height = 1.6in]{DeGPR/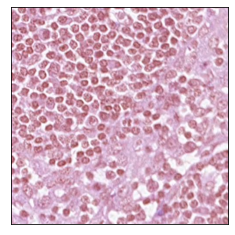}};
  
  \node[picture format,anchor=north west]                   (A2)   at (A1.north east)       {\includegraphics[width=1.6in, height = 1.6in]{DeGPR/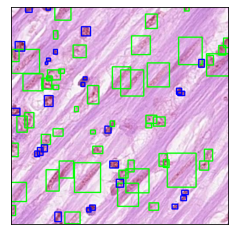}};
  \node[picture format,anchor=north]      (B2) at (A2.south) {\includegraphics[width=1.6in, height = 1.6in]{DeGPR/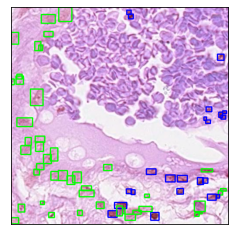}};
  \node[picture format,anchor=north]      (C2) at (B2.south) {\includegraphics[width=1.6in, height = 1.6in]{DeGPR/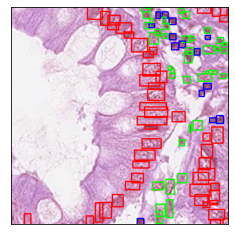}};
  \node[picture format,anchor=north]      (D2) at (C2.south) {\includegraphics[width=1.6in,  height = 1.6in]{DeGPR/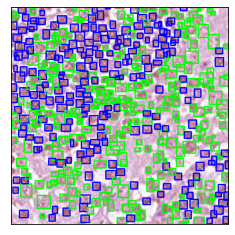}};

  \node[picture format,anchor=north west] (A3) at (A2.north east) {\includegraphics[width=1.6in, height = 1.6in]{DeGPR/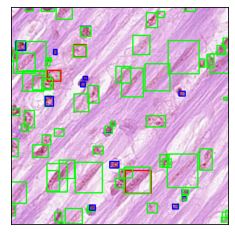}};
  \node[picture format,anchor=north]      (B3) at (A3.south)      {\includegraphics[width=1.6in, height = 1.6in]{DeGPR/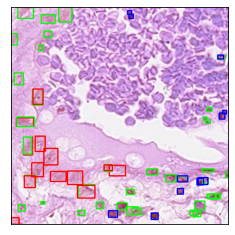}};
   \node[picture format,anchor=north]      (C3) at (B3.south)      {\includegraphics[width=1.6in, height=1.6in]{DeGPR/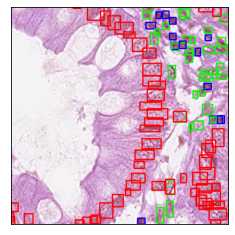}};
   \node[picture format,anchor=north]      (D3) at (C3.south)      {\includegraphics[width=1.6in, height = 1.6in]{DeGPR/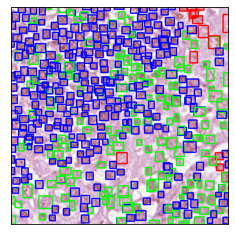}};

  \node[picture format,anchor=north west] (A4) at (A3.north east) {\includegraphics[width=1.6in, height = 1.6in]{DeGPR/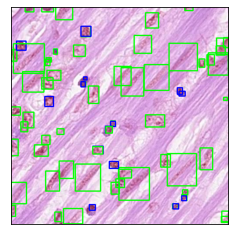}};
  \node[picture format,anchor=north]      (B4) at (A4.south)      {\includegraphics[width=1.6in, height = 1.6in]{DeGPR/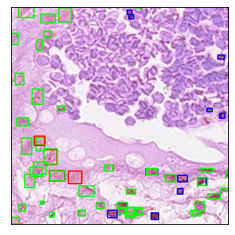}};
  \node[picture format,anchor=north]      (C4) at (B4.south)      {\includegraphics[width=1.6in, height=1.6in]{DeGPR/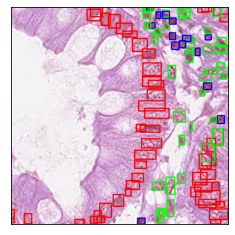}};
  \node[picture format,anchor=north]      (D4) at (C4.south)      {\includegraphics[width=1.6in, height = 1.6in]{DeGPR/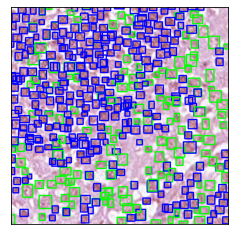}};
  %% Captions

  \node[anchor=south] (C1) at (A1.north) {\bfseries Original};
  \node[anchor=south] (C2) at (A2.north) {\bfseries Ground Truth};
  \node[anchor=south] (C3) at (A3.north) {\bfseries Baseline};
  \node[anchor=south] (C4) at (A4.north) {\bfseries Proposed};

\end{tikzpicture}
\caption{Qualitative performance of \sys{} for CoNSeP. The cells are marked as Blue (Inflammatory), Red (Epithelial) and Green (Spindle). We can see that the baseline model often misclassifies spindle cells as inflammatory cells. This is probably because of their high structural similarity. The model with \sys{} is successfully able to capture the differences between spindle and inflammatory cells. However, it is still not perfect as can be seen in row 4 where there are multiple misclassifications of spindle cells as epithelial cells. We believe one of the main reasons this happened is because of the high density of cells in the image and which dampens the effect of \sys{} since it considers the average feature difference between two classes}
\label{fig: bbox_prediction_CoNSeP}
\end{figure*}

\begin{figure*}
\centering
\begin{tikzpicture}[scale=1.03,transform shape, picture format/.style={inner sep=1pt}]

  \node[picture format]                   (A1)   at (0,0)            {\includegraphics[width=1.6in, height = 1.6in]{DeGPR/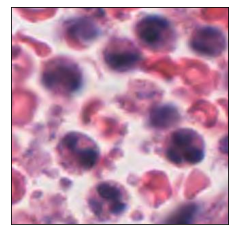}};
  \node[picture format,anchor=north]      (B1) at (A1.south) {\includegraphics[width=1.6in, height = 1.6in]{DeGPR/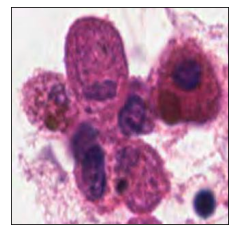}};
  \node[picture format,anchor=north]      (C1) at (B1.south) {\includegraphics[width=1.6in, height = 1.6in]{DeGPR/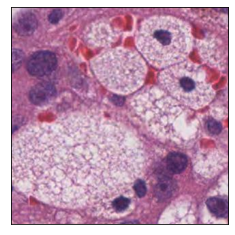}};
  \node[picture format,anchor=north]      (D1) at (C1.south) {\includegraphics[width=1.6in, height = 1.6in]{DeGPR/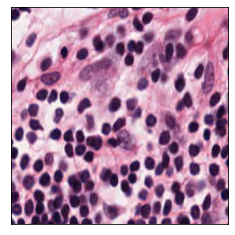}};
  
  \node[picture format,anchor=north west]                   (A2)   at (A1.north east)       {\includegraphics[width=1.6in, height = 1.6in]{DeGPR/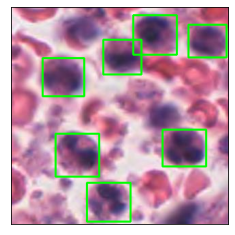}};
  \node[picture format,anchor=north]      (B2) at (A2.south) {\includegraphics[width=1.6in, height = 1.6in]{DeGPR/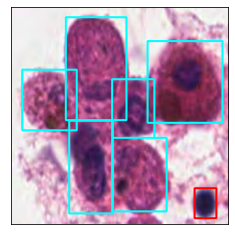}};
  \node[picture format,anchor=north]      (C2) at (B2.south) {\includegraphics[width=1.6in, height = 1.6in]{DeGPR/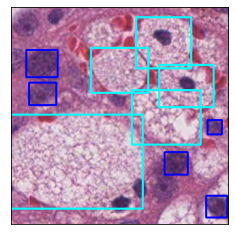}};
  \node[picture format,anchor=north]      (D2) at (C2.south) {\includegraphics[width=1.6in,  height = 1.6in]{DeGPR/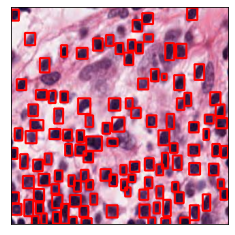}};

  \node[picture format,anchor=north west] (A3) at (A2.north east) {\includegraphics[width=1.6in, height = 1.6in]{DeGPR/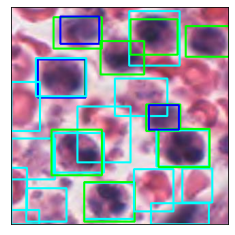}};
  \node[picture format,anchor=north]      (B3) at (A3.south)      {\includegraphics[width=1.6in, height = 1.6in]{DeGPR/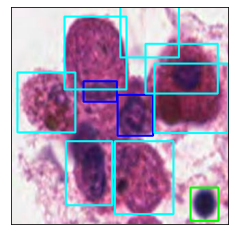}};
   \node[picture format,anchor=north]      (C3) at (B3.south)      {\includegraphics[width=1.6in, height=1.6in]{DeGPR/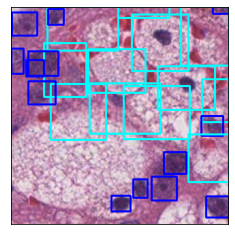}};
   \node[picture format,anchor=north]      (D3) at (C3.south)      {\includegraphics[width=1.6in, height = 1.6in]{DeGPR/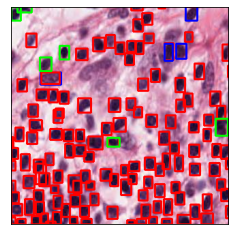}};

  \node[picture format,anchor=north west] (A4) at (A3.north east) {\includegraphics[width=1.6in, height = 1.6in]{DeGPR/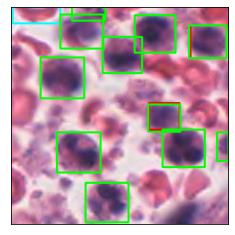}};
  \node[picture format,anchor=north]      (B4) at (A4.south)      {\includegraphics[width=1.6in, height = 1.6in]{DeGPR/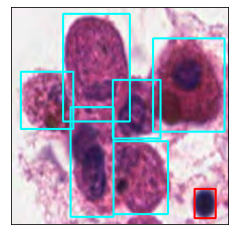}};
  \node[picture format,anchor=north]      (C4) at (B4.south)      {\includegraphics[width=1.6in, height=1.6in]{DeGPR/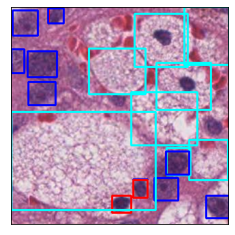}};
  \node[picture format,anchor=north]      (D4) at (C4.south)      {\includegraphics[width=1.6in, height = 1.6in]{DeGPR/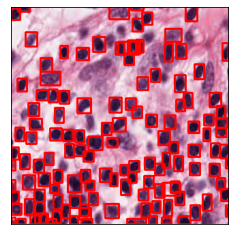}};
  %% Captions

  \node[anchor=south] (C1) at (A1.north) {\bfseries Original};
  \node[anchor=south] (C2) at (A2.north) {\bfseries Ground Truth};
  \node[anchor=south] (C3) at (A3.north) {\bfseries Baseline};
  \node[anchor=south] (C4) at (A4.north) {\bfseries Proposed};

\end{tikzpicture}
\caption{Qualitative performance of \sys{} for MoNuSAC. The cells are marked as Blue (Epithelial), Red (Lymphocyte), Green (Neutrophil) and Cyan (Macrophage). The baseline model often makes extra predictions for the macrophage class as is evident from the first three rows. The model with \sys{} is able to successfully solve this issue. In row 3, we can also see how the model with \sys{} is able to detect the large macrophage which was missed by the baseline model. This is a perfect example where size as an explicit feature is helping the model. In row 2 and row 4, the baseline model misclassifies lymphocytes as epithelial or neutrophil cells. The model with \sys{} is successfully able to solve this issue. At the same time, there are some errors like extra predictions in rows 1 and 3. These extra predictions probably arise since the detected cells are structurally similar to our required cells.}
\label{fig: bbox_prediction_MoNuSAC}
\end{figure*}

% {\small
% \bibliographystyle{ieee_fullname}
% \bibliography{egbib}
% }

\end{document}
